# Supplementary material for: Validation of satellite and reanalysis rainfall products against rain gauge observations in Ghana and Zambia
Source: arXiv:2501.14829 source file (2025-04-11)
Supplement: Supplementary file 1 [file Supplementary_Material.pdf]

# Supplementary Material for Validation of satellite and reanalysis rainfall products against rain gauge observations in Ghana and Zambia

John Bagiliko, David Stern, Denis Ndanguza, Francis Feehi Torgbor

Corresponding author: John Bagiliko, john.bagiliko@aims-senegal.org

## Ombrothermic Diagrams of the Stations in Ghana and Zambia

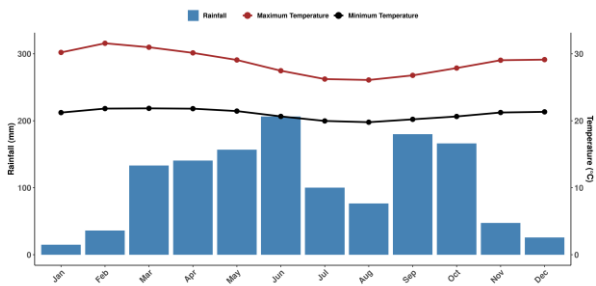

**Fig. E1: Ombrothermic diagram of Abetifi, Ghana.**

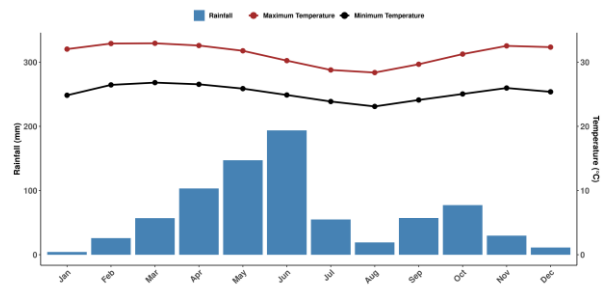

**Fig. E2: Ombrothermic diagram of Ada, Ghana.**

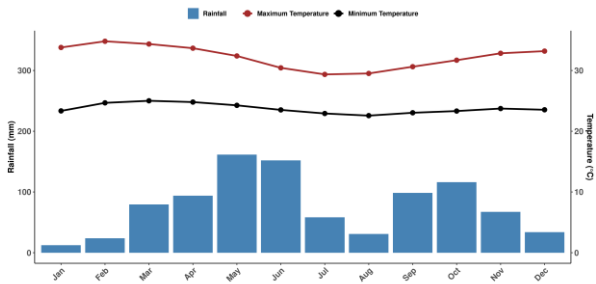

**Fig. E3: Ombrothermic diagram of Akatsi, Ghana.**

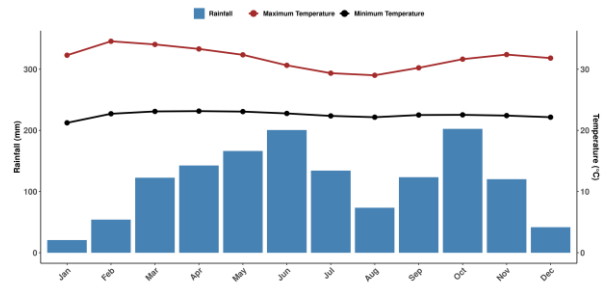

**Fig. E4: Ombrothermic diagram of Akim Oda, Ghana.**

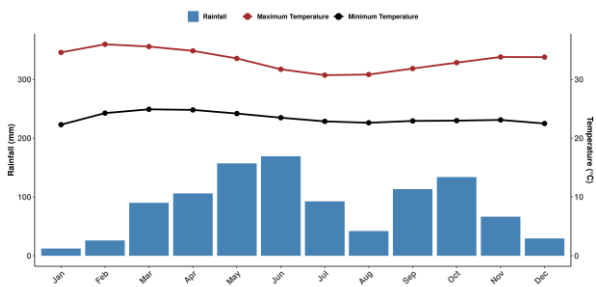

**Fig. E5: Ombrothermic diagram of Akuse, Ghana.**

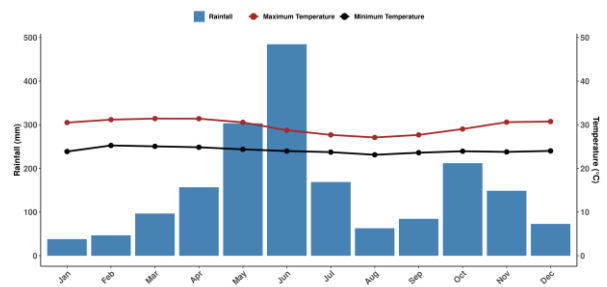

**Fig. E6: Ombrothermic diagram of Axim, Ghana.**

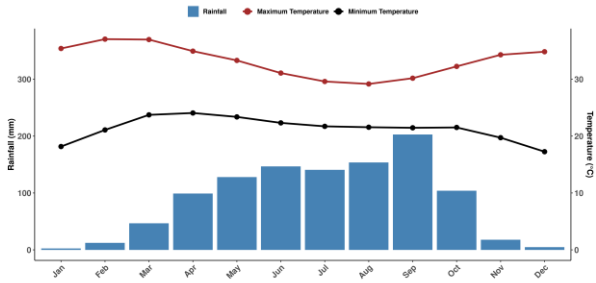

**Fig. E7: Ombrothermic diagram of Bole, Ghana.**

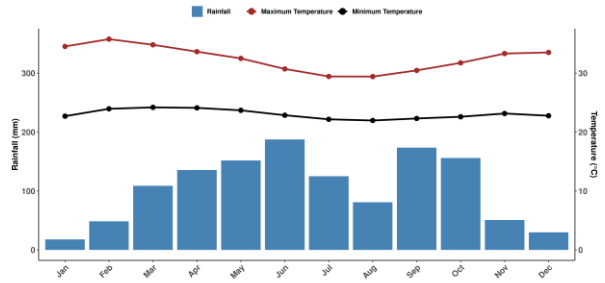

**Fig. E8: Ombrothermic diagram of Ho, Ghana.**

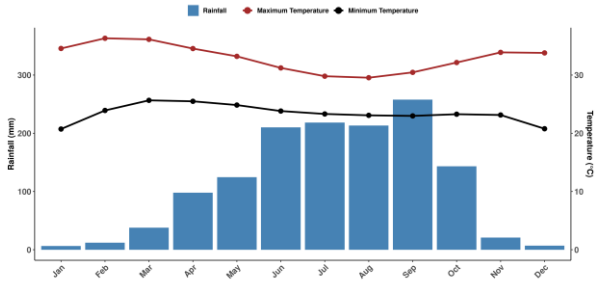

**Fig. E9: Ombrothermic diagram of Kete-Krachi, Ghana.**

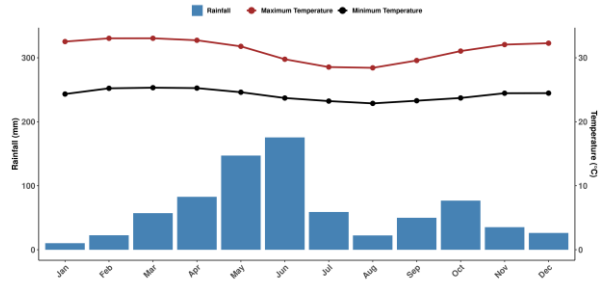

**Fig. E10: Ombrothermic diagram of KIAMO-Accra, Ghana.**

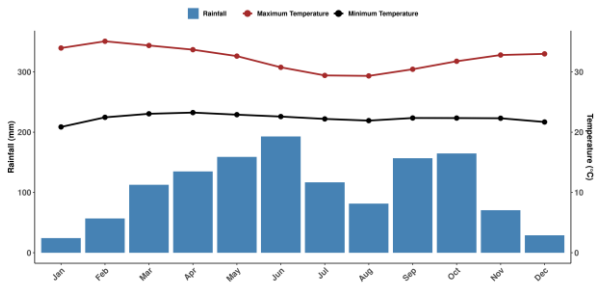

**Fig. E11: Ombrothermic diagram of Koforidua, Ghana.**

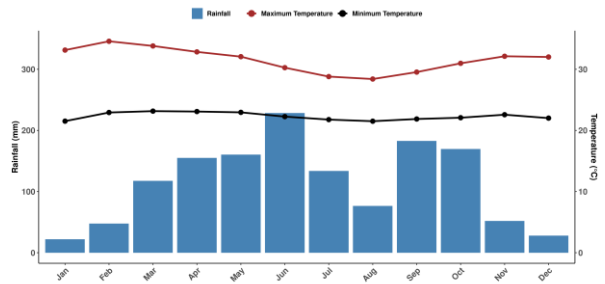

**Fig. E12: Ombrothermic diagram of Kumasi, Ghana.**

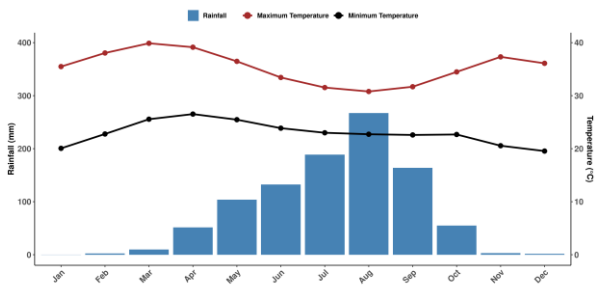

**Fig. E13: Ombrothermic diagram of Navrogo, Ghana.**

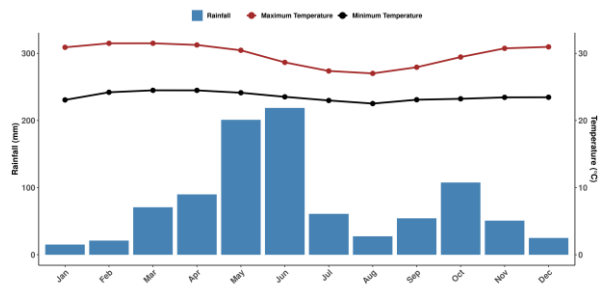

**Fig. E14: Ombrothermic diagram of Saltpond, Ghana.**

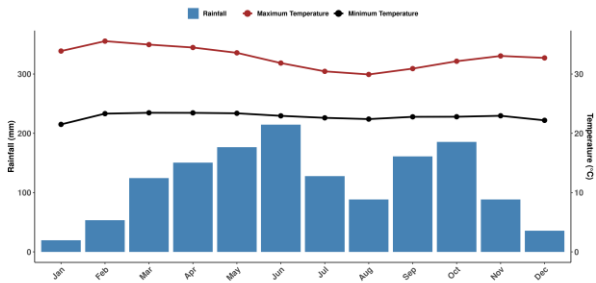

**Fig. E15: Ombrothermic diagram of Sefwi Bekwai, Ghana.**

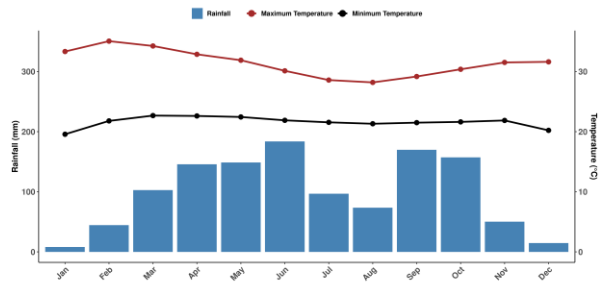

**Fig. E16: Ombrothermic diagram of Sunyani, Ghana.**

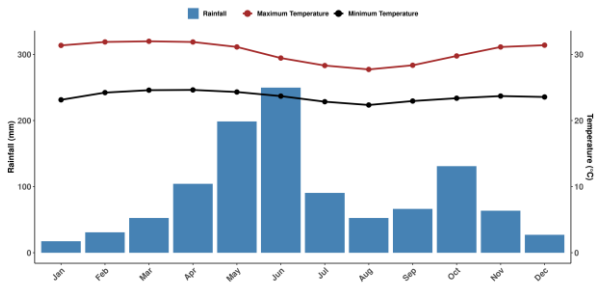

**Fig. E17: Ombrothermic diagram of Takoradi, Ghana.**

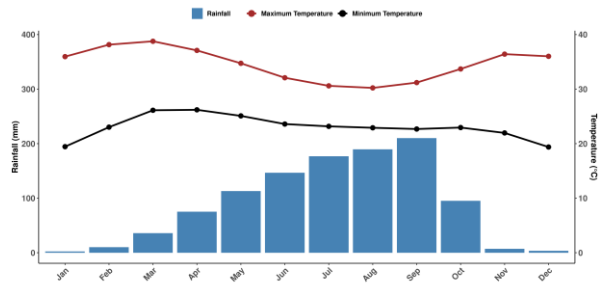

**Fig. E18: Ombrothermic diagram of Tamale, Ghana.**

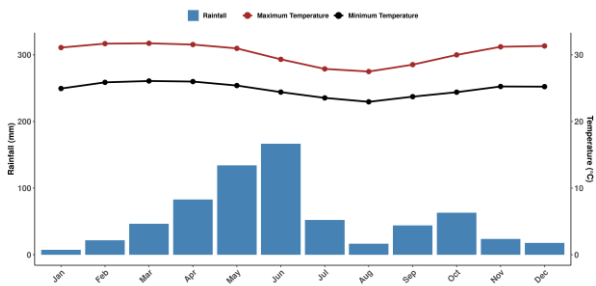

**Fig. E19: Ombrothermic diagram of Tema, Ghana.**

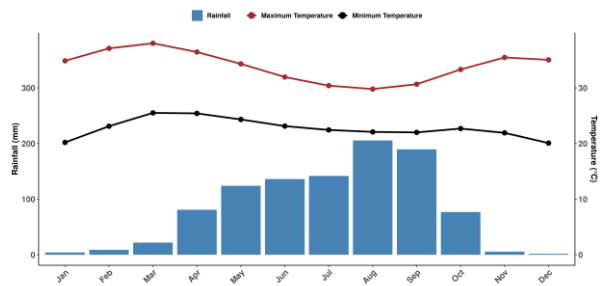

**Fig. E20: Ombrothermic diagram of Wa, Ghana.**

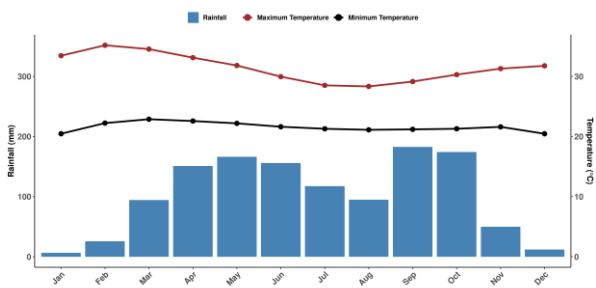

**Fig. E21: Ombrothermic diagram of Wenchi, Ghana.**

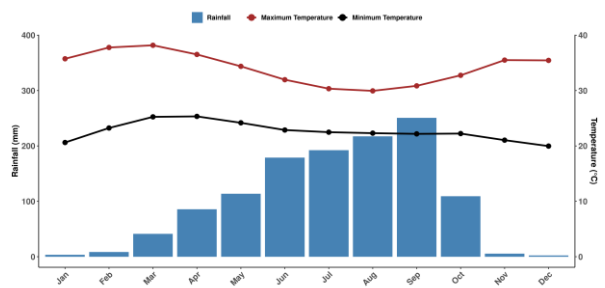

**Fig. E22: Ombrothermic diagram of Yendi, Ghana.**

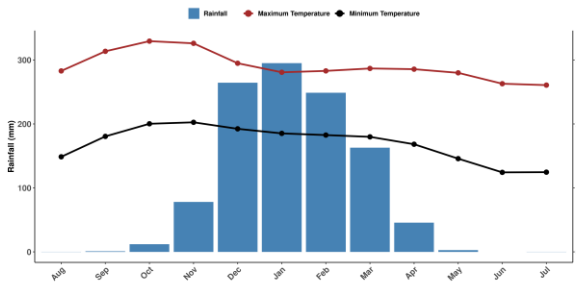

**Fig. E23: Ombrothermic diagram of Chipata, Zambia.**

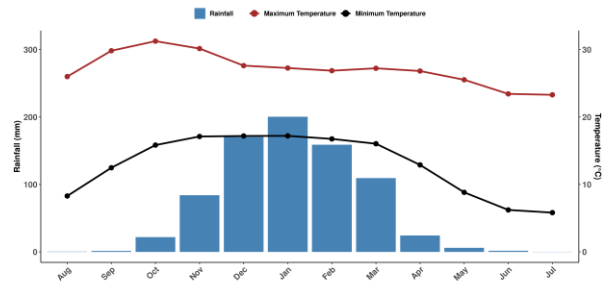

**Fig. E24: Ombrothermic diagram of Choma, Zambia.**

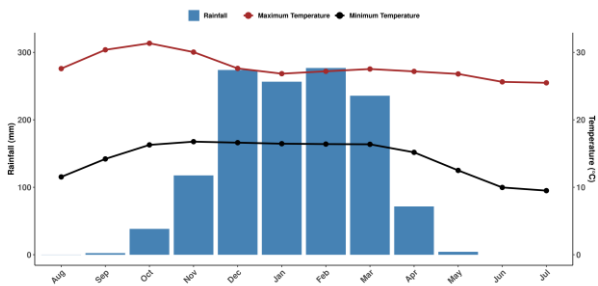

**Fig. E25: Ombrothermic diagram of Kasama, Zambia.**

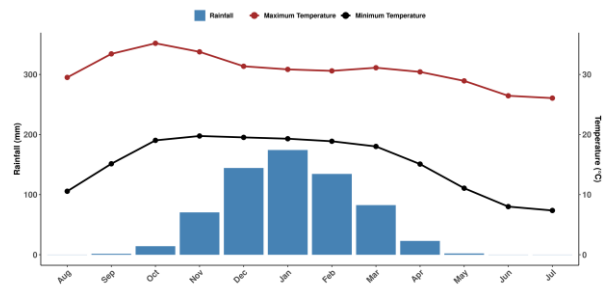

**Fig. E26: Ombrothermic diagram of Livingstone, Zambia.**

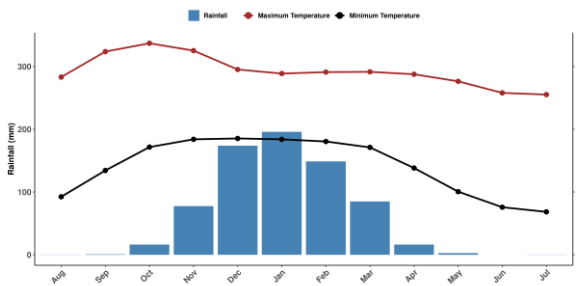

**Fig. E27: Ombrothermic diagram of Magoye, Zambia.**

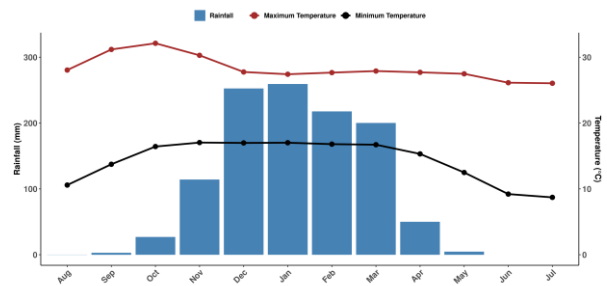

**Fig. E28: Ombrothermic diagram of Magoye, Zambia.**

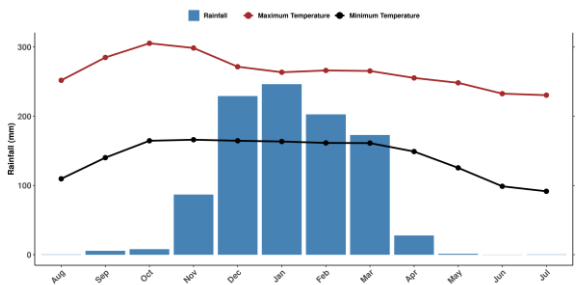

**Fig. E29: Ombrothermic diagram of Mpika, Zambia.**

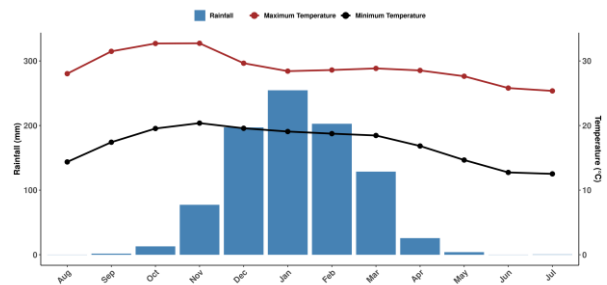

**Fig. E30: Ombrothermic diagram of Petauke, Zambia.**

Annual Total Rainfall – Zambia

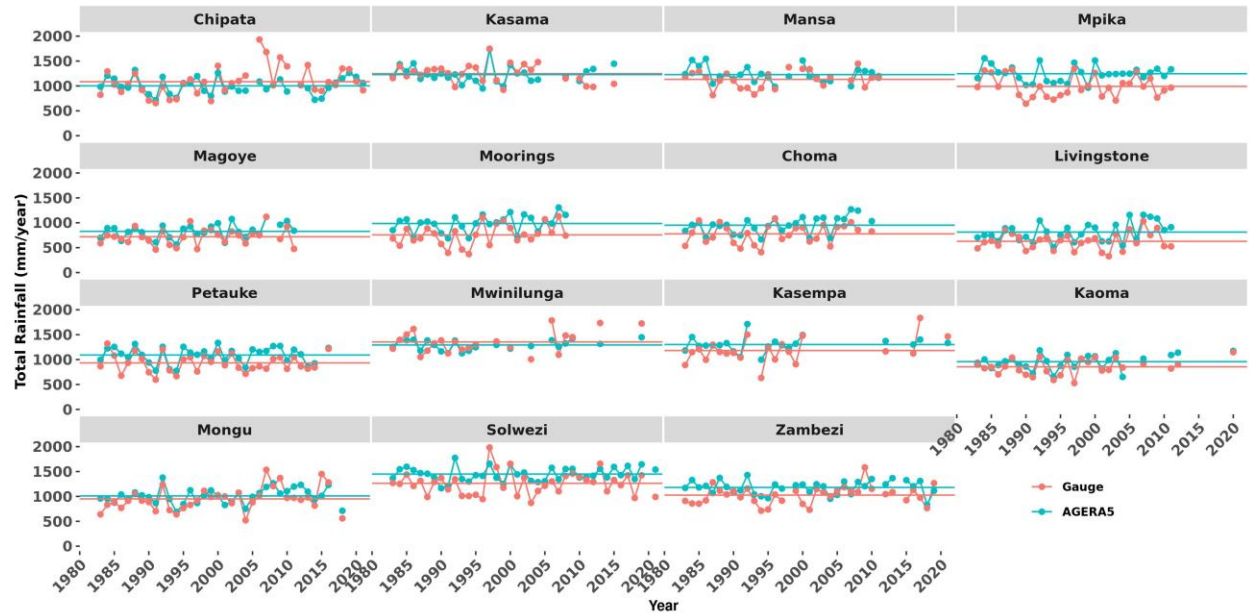

**Fig E31: Total annual rainfall across the stations in Zambia – rain gauge vs AGERA5. The horizontal lines represent mean annual total rainfall across all the years considered for the gauge (red) and the AGERA5 (blue).**

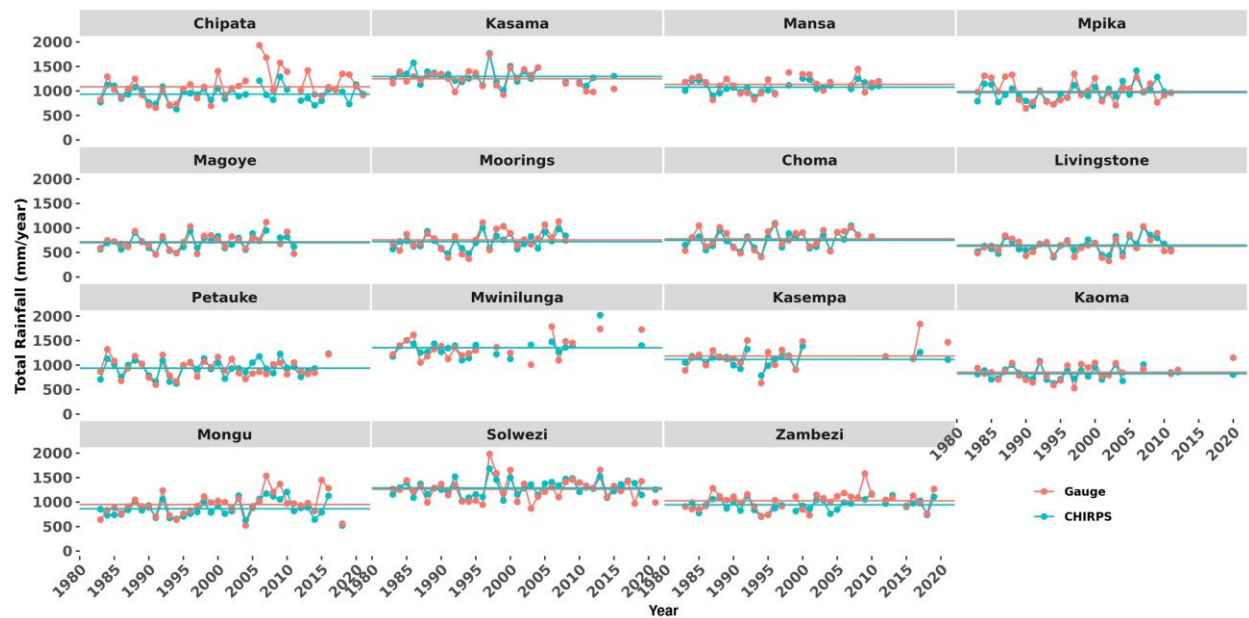

**Fig E32: Total annual rainfall across the stations in Zambia – rain gauge vs CHIRPS. The horizontal lines represent mean annual total rainfall across all the years considered for the gauge (red) and the CHIRPS (blue).**

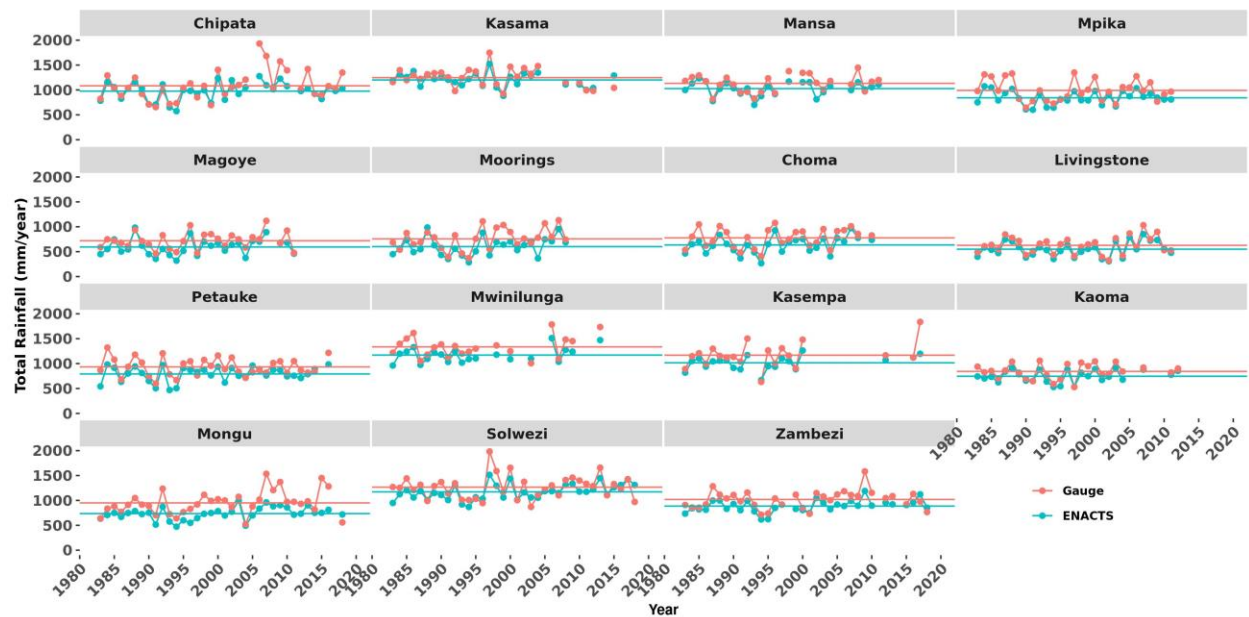

**Fig E33: Total annual rainfall across the stations in Zambia – rain gauge vs ENACTS. The horizontal lines represent mean annual total rainfall across all the years considered for the gauge (red) and the ENACTS (blue).**

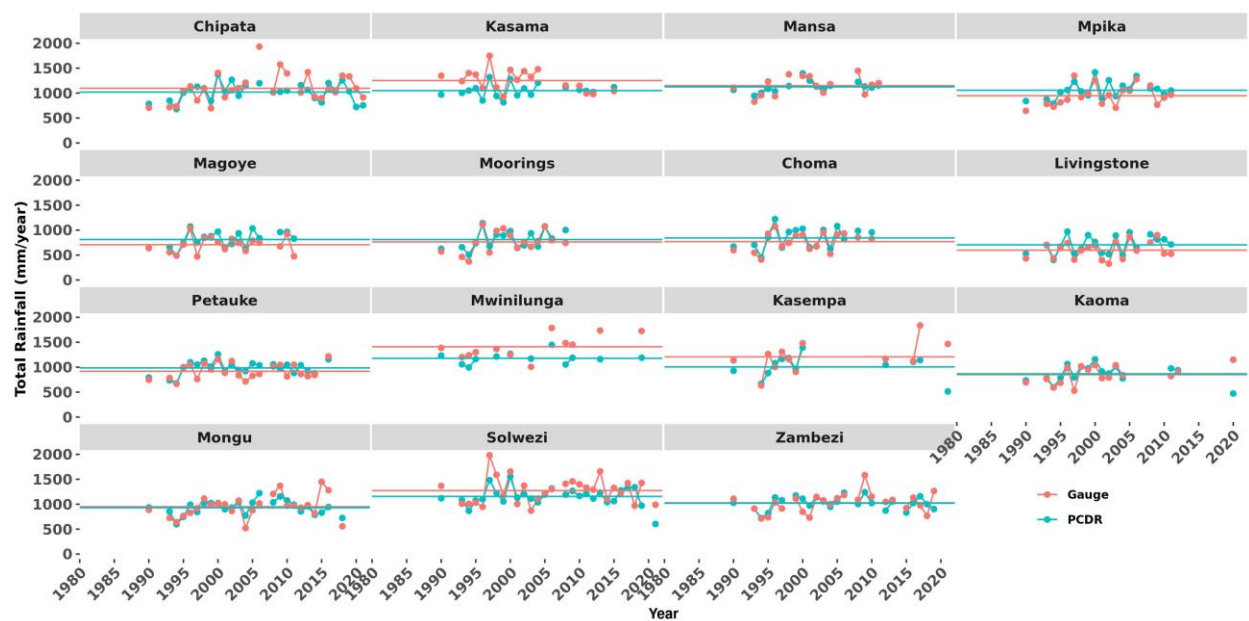

**Fig E34: Total annual rainfall across the stations in Zambia – rain gauge vs PCDR. The horizontal lines represent mean annual total rainfall across all the years considered for the gauge (red) and the PCDR (blue).**

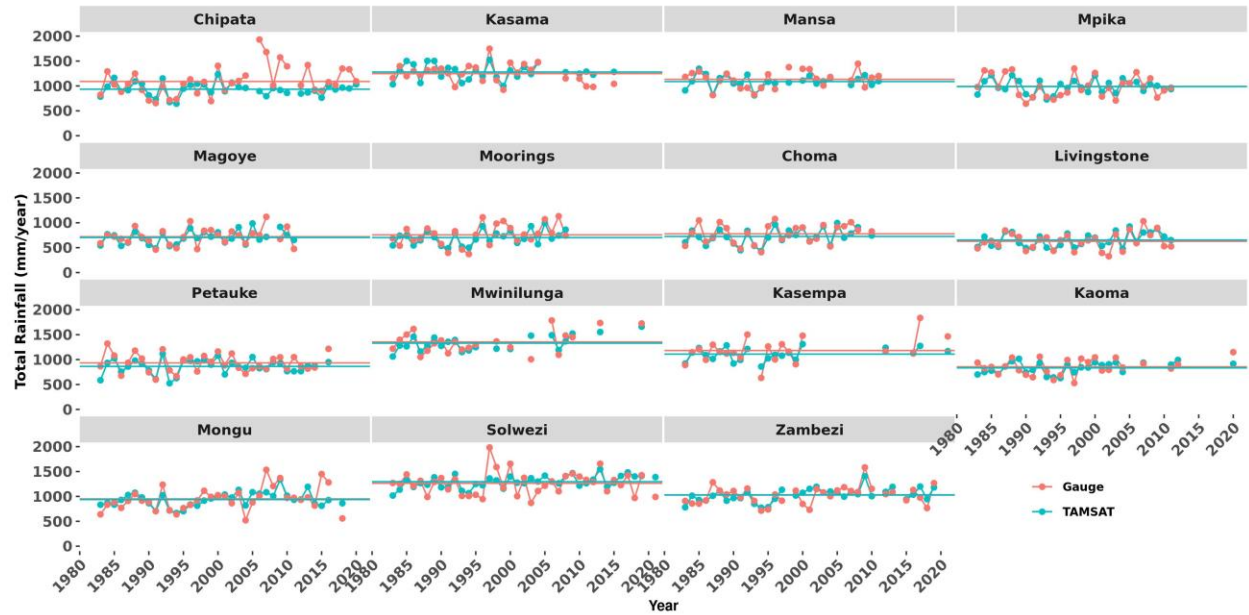

**Fig E35: Total annual rainfall across the stations in Zambia – rain gauge vs TAMSAT. The horizontal lines represent mean annual total rainfall across all the years considered for the gauge (red) and the TAMSAT (blue).**

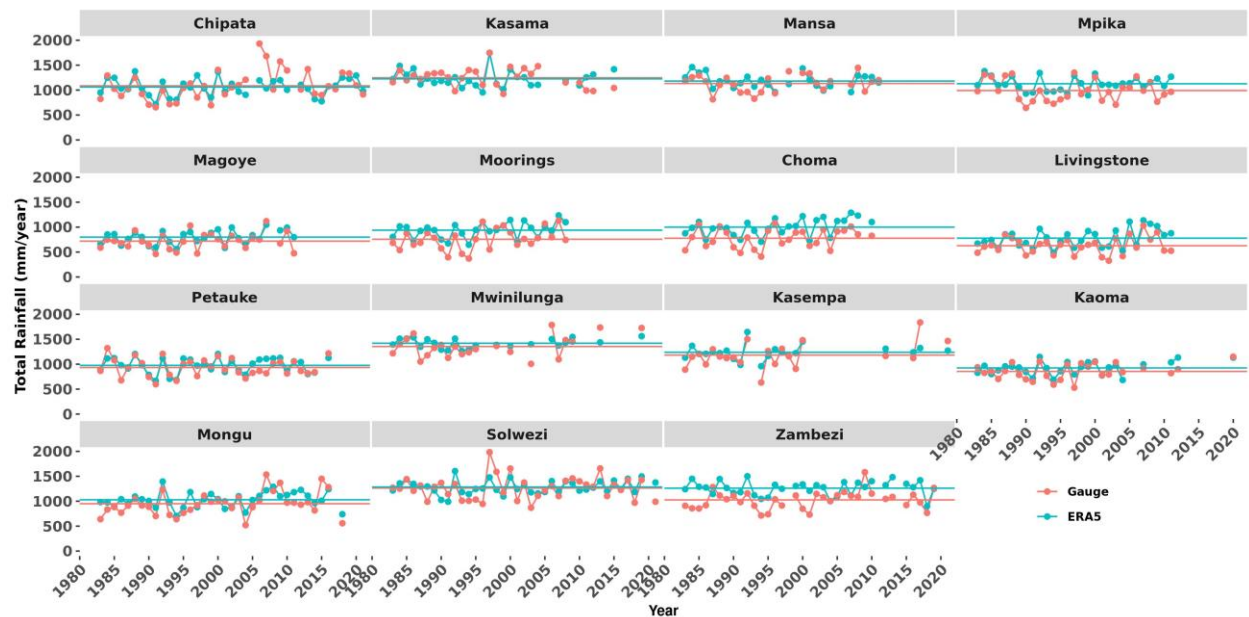

**Fig E36: Total annual rainfall across the stations in Zambia – rain gauge vs ERA5. The horizontal lines represent mean annual total rainfall across all the years considered for the gauge (red) and the ERA5 (blue).**

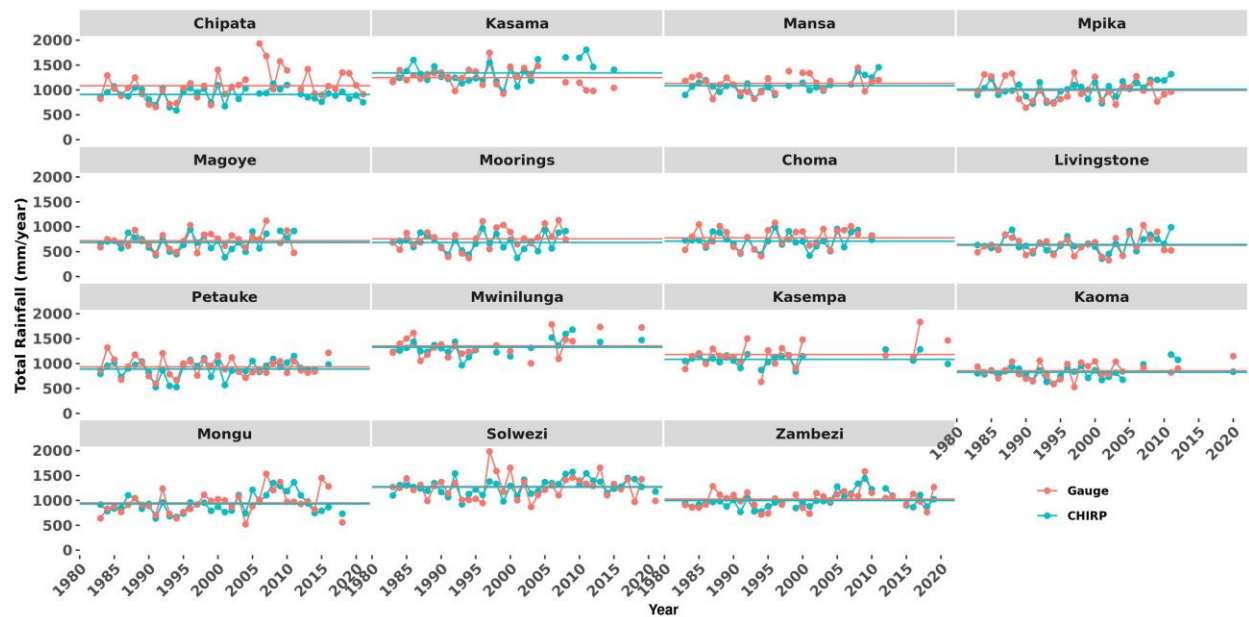

**Fig E37: Total annual rainfall across the stations in Zambia – rain gauge vs CHIRP. The horizontal lines represent mean annual total rainfall across all the years considered for the gauge (red) and the CHIRP (blue).**

**Table E1: Summary statistics on the performance of the products on annual total rainfall**

| Metric | station     | CHIRPS | CHIRP | ENACTS | ERA5 | PCDR | TAMSAT | AGERA5 |
|--------|-------------|--------|-------|--------|------|------|--------|--------|
| r      | Chipata     | 0.61   | 0.49  | 0.8    | 0.54 | 0.57 | 0.27   | 0.47   |
| r      | Kasama      | 0.79   | 0.12  | 0.81   | 0.42 | 0.68 | 0.47   | 0.43   |
| r      | Mansa       | 0.76   | 0.43  | 0.84   | 0.48 | 0.79 | 0.5    | 0.44   |
| r      | Mpika       | 0.59   | 0.46  | 0.89   | 0.69 | 0.82 | 0.69   | 0.68   |
| r      | Magoye      | 0.87   | 0.46  | 0.87   | 0.76 | 0.7  | 0.59   | 0.74   |
| r      | Moorings    | 0.84   | 0.66  | 0.8    | 0.72 | 0.82 | 0.7    | 0.7    |
| r      | Choma       | 0.9    | 0.68  | 0.93   | 0.8  | 0.9  | 0.8    | 0.77   |
| r      | Livingstone | 0.9    | 0.63  | 0.97   | 0.82 | 0.83 | 0.78   | 0.81   |

|              |             |      |      |      |      |      |      |      |
|--------------|-------------|------|------|------|------|------|------|------|
| <b>r</b>     | Petauke     | 0.72 | 0.56 | 0.75 | 0.78 | 0.69 | 0.66 | 0.77 |
| <b>r</b>     | Mwinilunga  | 0.6  | 0.58 | 0.93 | 0.61 | 0.44 | 0.63 | 0.64 |
| <b>r</b>     | Kasempa     | 0.75 | 0.63 | 0.85 | 0.63 | 0.31 | 0.67 | 0.63 |
| <b>r</b>     | Kaoma       | 0.72 | 0.41 | 0.89 | 0.71 | 0.35 | 0.62 | 0.74 |
| <b>r</b>     | Mongu       | 0.74 | 0.5  | 0.74 | 0.67 | 0.58 | 0.58 | 0.67 |
| <b>r</b>     | Solwezi     | 0.68 | 0.52 | 0.77 | 0.52 | 0.6  | 0.39 | 0.51 |
| <b>r</b>     | Zambezi     | 0.66 | 0.63 | 0.78 | 0.31 | 0.57 | 0.62 | 0.33 |
| <b>PBIAS</b> | Chipata     | -14  | -16  | -10  | -2   | -7   | -14  | -8   |
| <b>PBIAS</b> | Kasama      | 4    | 8    | -4   | -2   | -16  | 3    | -2   |
| <b>PBIAS</b> | Mansa       | -5   | -4   | -9   | 4    | -2   | -4   | 8    |
| <b>PBIAS</b> | Mpika       | -2   | 2    | -15  | 14   | 12   | 0    | 26   |
| <b>PBIAS</b> | Magoye      | -2   | -5   | -17  | 11   | 15   | -2   | 15   |
| <b>PBIAS</b> | Moorings    | -5   | -10  | -20  | 24   | 6    | -7   | 30   |
| <b>PBIAS</b> | Choma       | -4   | -8   | -18  | 29   | 10   | -7   | 22   |
| <b>PBIAS</b> | Livingstone | 4    | 2    | -12  | 24   | 18   | 4    | 30   |
| <b>PBIAS</b> | Petauke     | 0    | -5   | -15  | 4    | 7    | -8   | 17   |
| <b>PBIAS</b> | Mwinilunga  | 0    | -2   | -12  | 5    | -16  | -2   | -4   |

|              |             |      |      |      |      |      |      |      |
|--------------|-------------|------|------|------|------|------|------|------|
| <b>PBIAS</b> | Kasempa     | -6   | -8   | -13  | 5    | -17  | -6   | 10   |
| <b>PBIAS</b> | Kaoma       | -4   | -3   | -12  | 8    | 2    | -2   | 12   |
| <b>PBIAS</b> | Mongu       | -9   | -2   | -23  | 8    | -2   | -1   | 6    |
| <b>PBIAS</b> | Solwezi     | 2    | 1    | -8   | 2    | -9   | 3    | 15   |
| <b>PBIAS</b> | Zambezi     | -8   | -3   | -13  | 23   | -1   | 0    | 15   |
| <b>RSD</b>   | Chipata     | 0.54 | 0.48 | 0.6  | 0.59 | 0.62 | 0.46 | 0.56 |
| <b>RSD</b>   | Kasama      | 0.86 | 1.1  | 0.74 | 0.9  | 0.61 | 0.81 | 0.9  |
| <b>RSD</b>   | Mansa       | 0.63 | 0.89 | 0.79 | 0.83 | 0.6  | 0.74 | 0.9  |
| <b>RSD</b>   | Mpika       | 0.79 | 0.78 | 0.64 | 0.64 | 0.82 | 0.64 | 0.74 |
| <b>RSD</b>   | Magoye      | 0.83 | 0.96 | 0.99 | 0.81 | 1.03 | 0.8  | 0.88 |
| <b>RSD</b>   | Moorings    | 0.72 | 0.78 | 0.86 | 0.74 | 0.85 | 0.69 | 0.8  |
| <b>RSD</b>   | Choma       | 0.9  | 0.85 | 0.89 | 0.89 | 1.11 | 0.82 | 0.87 |
| <b>RSD</b>   | Livingstone | 0.87 | 0.93 | 0.86 | 1.06 | 1.04 | 0.84 | 1.1  |
| <b>RSD</b>   | Petauke     | 0.92 | 0.93 | 0.82 | 0.85 | 0.89 | 0.8  | 0.9  |
| <b>RSD</b>   | Mwinilunga  | 0.86 | 0.73 | 0.7  | 0.42 | 0.49 | 0.7  | 0.45 |
| <b>RSD</b>   | Kasempa     | 0.55 | 0.46 | 0.56 | 0.58 | 0.78 | 0.5  | 0.59 |
| <b>RSD</b>   | Kaoma       | 0.77 | 0.86 | 0.81 | 0.84 | 1.01 | 0.72 | 0.94 |

|            |             |         |         |         |        |         |         |        |
|------------|-------------|---------|---------|---------|--------|---------|---------|--------|
| <b>RSD</b> | Mongu       | 0.74    | 0.83    | 0.54    | 0.67   | 0.63    | 0.62    | 0.67   |
| <b>RSD</b> | Solwezi     | 0.68    | 0.67    | 0.67    | 0.58   | 0.7     | 0.52    | 0.59   |
| <b>RSD</b> | Zambezi     | 0.71    | 0.89    | 0.69    | 0.79   | 0.67    | 0.75    | 0.76   |
| <b>ME</b>  | Chipata     | -151.57 | -176.37 | -106.88 | -24.2  | -76.85  | -156.41 | -84.2  |
| <b>ME</b>  | Kasama      | 48.1    | 94.15   | -47.24  | -22.14 | -201.14 | 31.89   | -18.69 |
| <b>ME</b>  | Mansa       | -56.17  | -47.62  | -106.51 | 48.04  | -23.39  | -44.7   | 94.91  |
| <b>ME</b>  | Mpika       | -22     | 23.77   | -148.95 | 135.98 | 109.5   | -3.95   | 254.81 |
| <b>ME</b>  | Magoye      | -17.89  | -34.12  | -125.26 | 79.04  | 104.39  | -15.83  | 108.49 |
| <b>ME</b>  | Moorings    | -35.69  | -72     | -155.2  | 181.74 | 48.52   | -54.94  | 229.18 |
| <b>ME</b>  | Choma       | -28.34  | -66.27  | -142.05 | 222.84 | 73.92   | -52.15  | 173.55 |
| <b>ME</b>  | Livingstone | 22.94   | 15.85   | -78.14  | 150.94 | 106.76  | 24.95   | 185.18 |
| <b>ME</b>  | Petauke     | 3.44    | -43.77  | -141.38 | 42.25  | 67.15   | -70.1   | 158.12 |
| <b>ME</b>  | Mwinilunga  | -0.68   | -26.68  | -165.45 | 65.6   | -232.56 | -24.24  | -59.83 |
| <b>ME</b>  | Kasempa     | -68.36  | -98.3   | -153.16 | 56.04  | -201.2  | -72.94  | 119.84 |
| <b>ME</b>  | Kaoma       | -31.05  | -29.29  | -97.61  | 69.53  | 16.99   | -21.2   | 102.79 |
| <b>ME</b>  | Mongu       | -86.4   | -20.37  | -214.66 | 79.02  | -20.62  | -12.4   | 59.51  |
| <b>ME</b>  | Solwezi     | 26.22   | 12.51   | -94.62  | 21.49  | -117.4  | 32.49   | 184.74 |

|    |         |        |        |         |       |      |      |        |
|----|---------|--------|--------|---------|-------|------|------|--------|
| ME | Zambezi | -81.77 | -29.26 | -133.01 | 234.8 | -7.3 | 4.56 | 154.21 |
|----|---------|--------|--------|---------|-------|------|------|--------|

## Annual Number of Rainy Days – Zambia

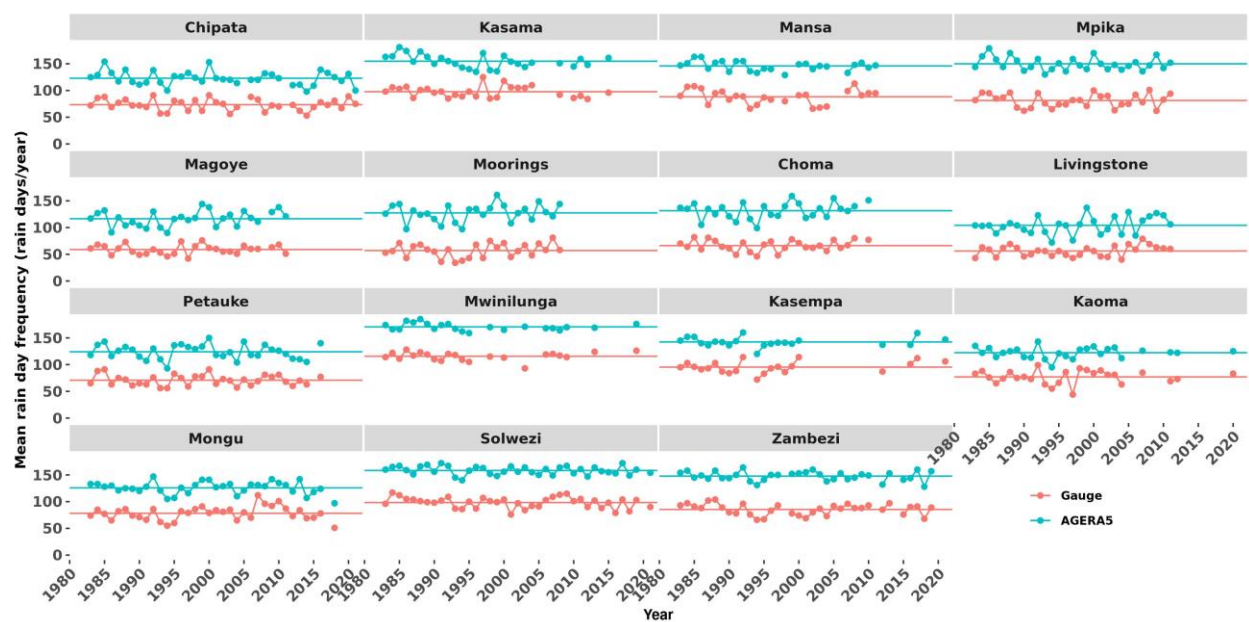

**Fig E38: Annual number of rainy days across the stations in Zambia – rain gauge vs AGERA. The horizontal lines represent mean number of rainy days across all the years considered for the gauge (red) and the CHIRP (blue).**

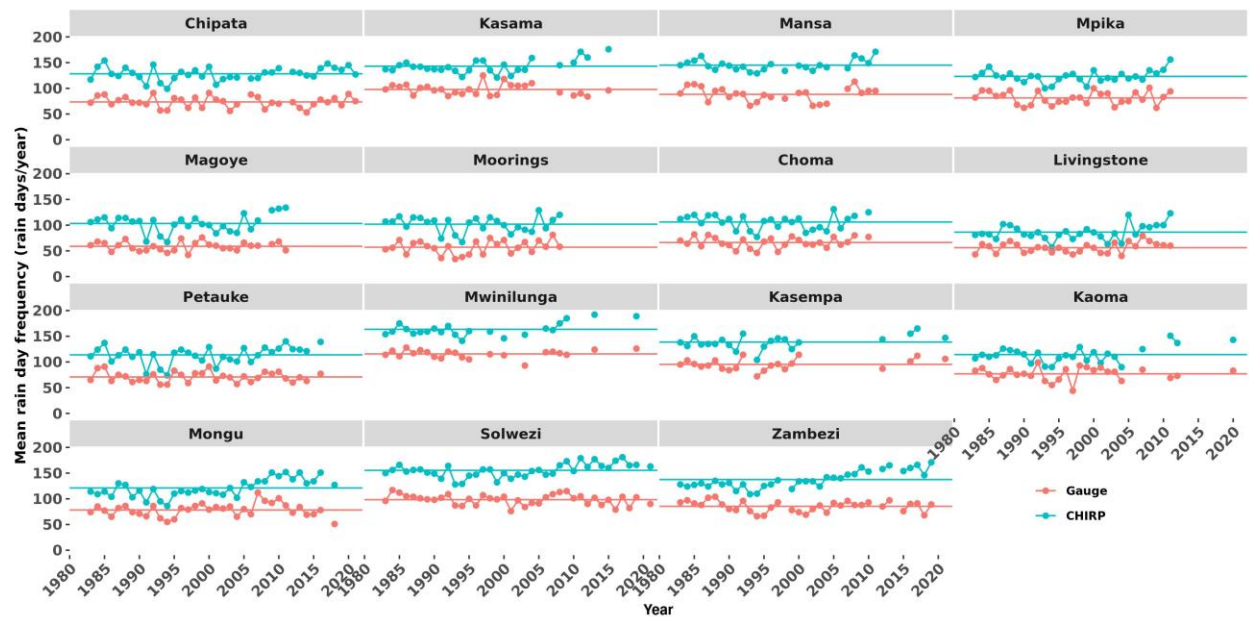

**Fig E39: Annual number of rainy days across the stations in Zambia – rain gauge vs CHIRP. The horizontal lines represent mean number of rainy days across all the years considered for the gauge (red) and the CHIRP (blue).**

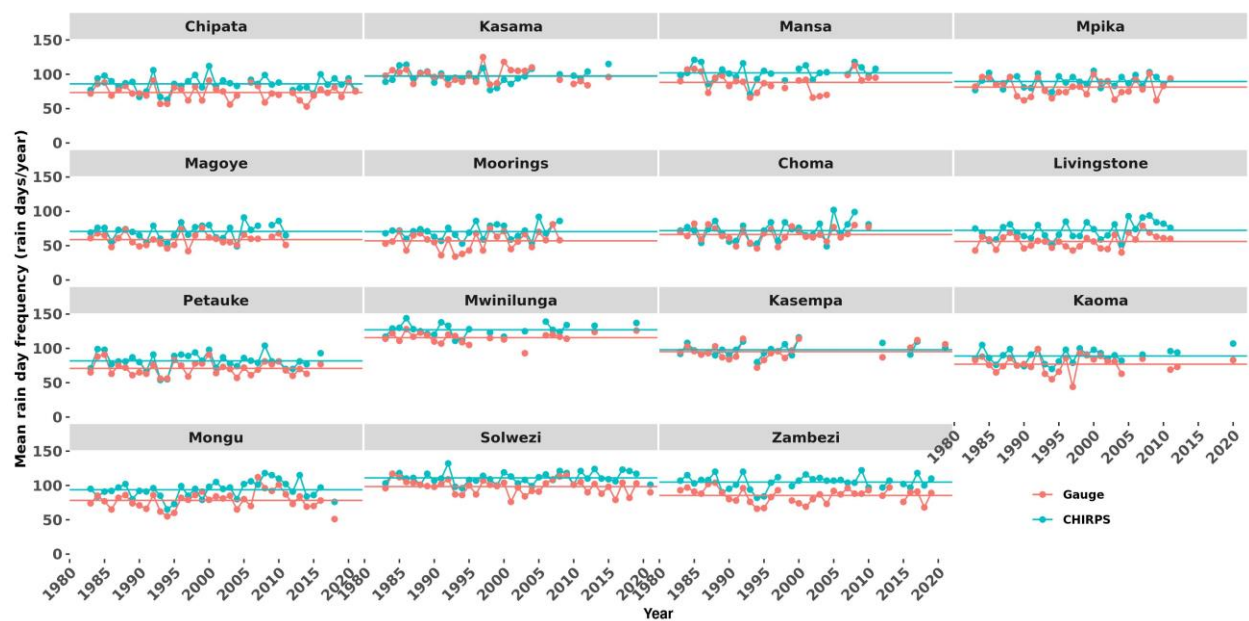

**Fig E40: Annual number of rainy days across the stations in Zambia – rain gauge vs CHIRPS. The horizontal lines represent mean number of rainy days across all the years considered for the gauge (red) and the CHIRPS (blue).**

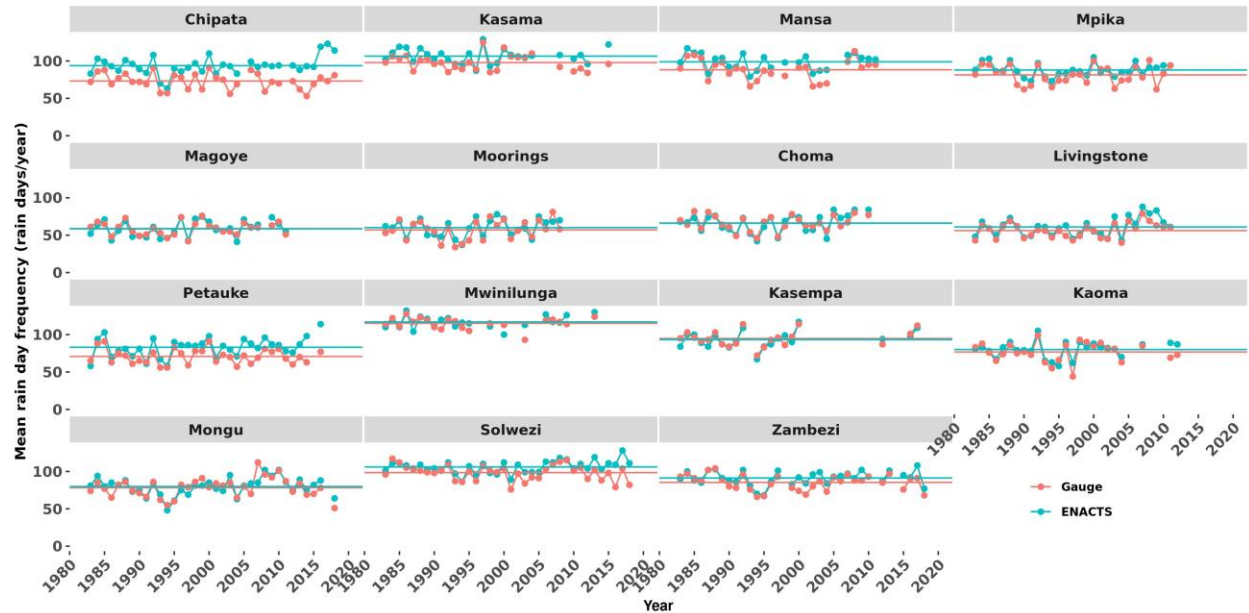

**Fig E41: Annual number of rainy days across the stations in Zambia – rain gauge vs ENACTS. The horizontal lines represent mean number of rainy days across all the years considered for the gauge (red) and the ENACTS (blue).**

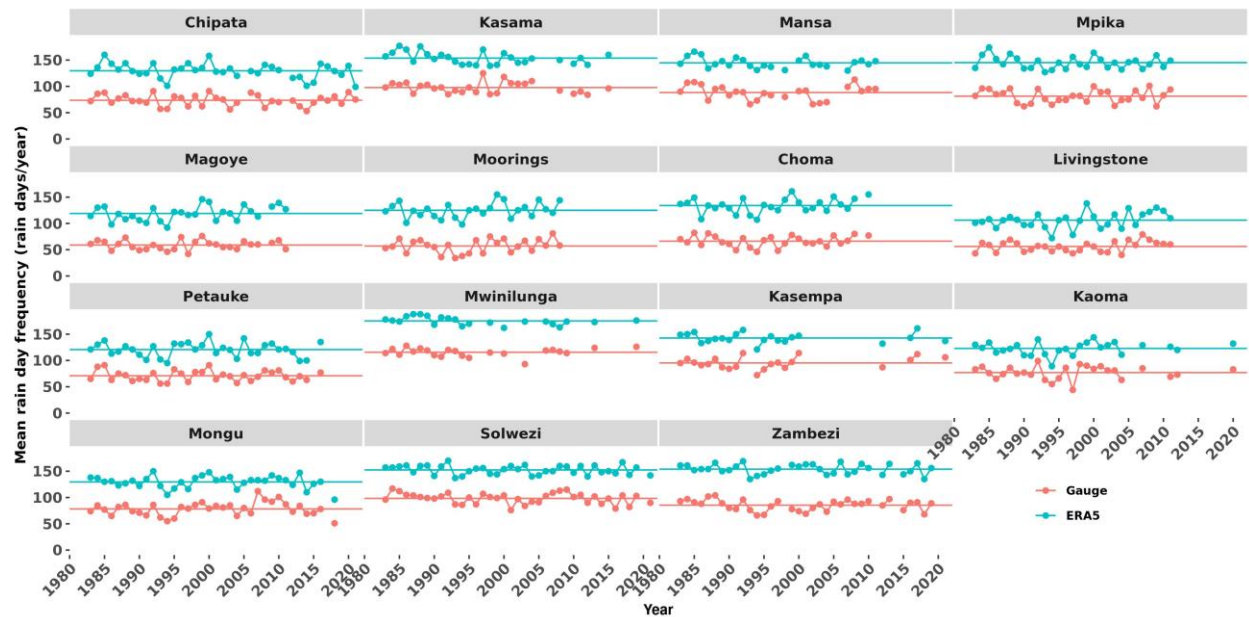

**Fig E42: Annual number of rainy days across the stations in Zambia – rain gauge vs ERA5. The horizontal lines represent mean number of rainy days across all the years considered for the gauge (red) and the ERA5 (blue).**

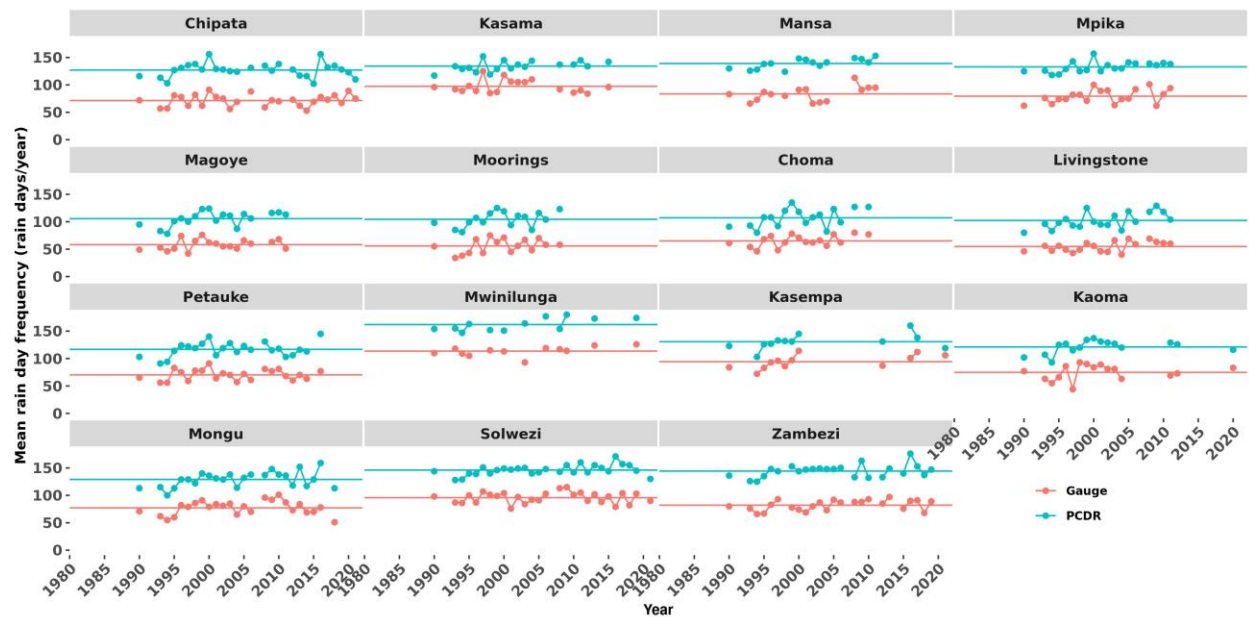

**Fig E43: Annual number of rainy days across the stations in Zambia – rain gauge vs PCDR. The horizontal lines represent mean number of rainy days across all the years considered for the gauge (red) and the PCDR (blue).**

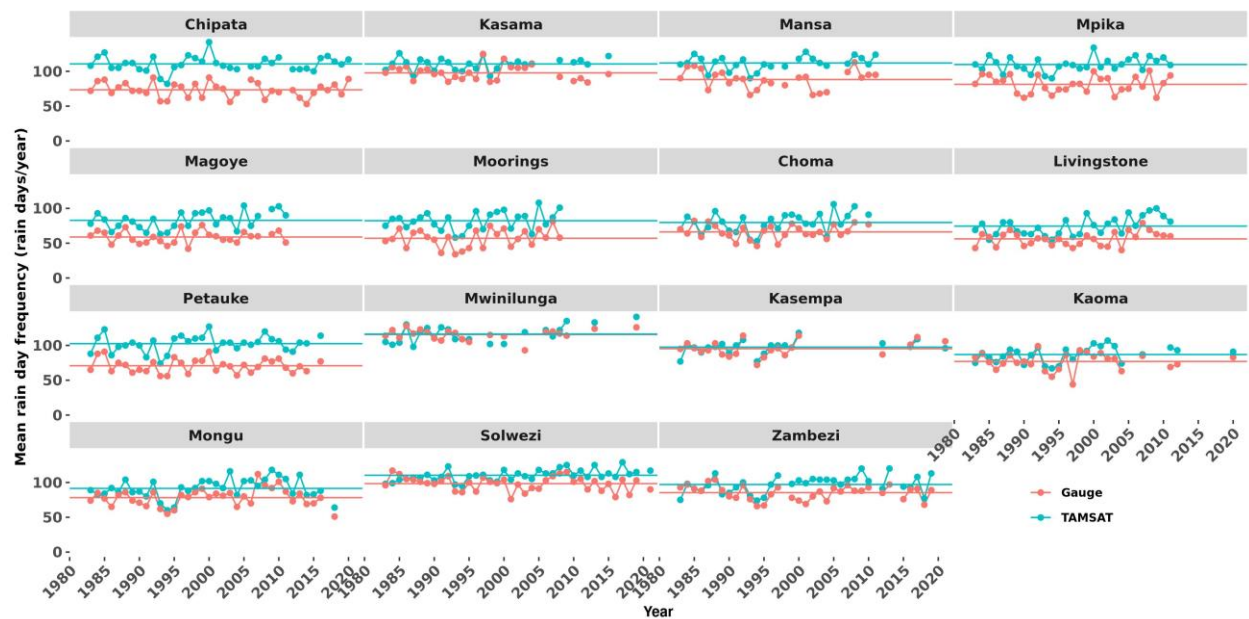

**Fig E44: Annual number of rainy days across the stations in Zambia – rain gauge vs TAMSAT. The horizontal lines represent mean number of rainy days across all the years considered for the gauge (red) and the TAMSAT (blue).**

**Table E2: Summary statistics on the performance of the products on annual number of rainy day**

| Metric | station | CHIRPS | CHIRP | ENACTS | ERA5 | PCDR | TAMSAT | AGERA5 |
|--------|---------|--------|-------|--------|------|------|--------|--------|
|--------|---------|--------|-------|--------|------|------|--------|--------|

|              |             |      |      |      |      |      |      |      |
|--------------|-------------|------|------|------|------|------|------|------|
| r            | Chipata     | 0.58 | 0.5  | 0.53 | 0.51 | 0.48 | 0.55 | 0.58 |
| r            | Kasama      | 0.37 | 0.05 | 0.74 | 0.63 | 0.58 | 0.54 | 0.57 |
| r            | Mansa       | 0.68 | 0.63 | 0.91 | 0.61 | 0.64 | 0.63 | 0.58 |
| r            | Mpika       | 0.5  | 0.56 | 0.79 | 0.48 | 0.59 | 0.56 | 0.46 |
| r            | Magoye      | 0.75 | 0.49 | 0.88 | 0.6  | 0.65 | 0.71 | 0.61 |
| r            | Moorings    | 0.77 | 0.74 | 0.81 | 0.64 | 0.81 | 0.8  | 0.66 |
| r            | Choma       | 0.76 | 0.8  | 0.88 | 0.77 | 0.88 | 0.71 | 0.76 |
| r            | Livingstone | 0.74 | 0.7  | 0.93 | 0.7  | 0.83 | 0.67 | 0.65 |
| r            | Petauke     | 0.77 | 0.59 | 0.69 | 0.72 | 0.7  | 0.81 | 0.78 |
| r            | Mwinilunga  | 0.32 | 0.4  | 0.46 | 0.33 | 0.3  | 0.3  | 0.44 |
| r            | Kasempa     | 0.62 | 0.63 | 0.87 | 0.7  | 0.63 | 0.67 | 0.79 |
| r            | Kaoma       | 0.69 | 0.28 | 0.83 | 0.73 | 0.55 | 0.62 | 0.74 |
| r            | Mongu       | 0.68 | 0.52 | 0.75 | 0.64 | 0.71 | 0.75 | 0.68 |
| r            | Solwezi     | 0.46 | 0.31 | 0.61 | 0.46 | 0.12 | 0.33 | 0.4  |
| r            | Zambezi     | 0.51 | 0.26 | 0.79 | 0.45 | 0.4  | 0.48 | 0.46 |
| <b>PBIAS</b> | Chipata     | 17   | 75   | 28   | 76   | 78   | 51   | 67   |
| <b>PBIAS</b> | Kasama      | 0    | 46   | 9    | 57   | 38   | 13   | 58   |

|              |             |      |      |      |      |      |      |      |
|--------------|-------------|------|------|------|------|------|------|------|
| <b>PBIAS</b> | Mansa       | 16   | 64   | 12   | 64   | 66   | 27   | 65   |
| <b>PBIAS</b> | Mpika       | 10   | 52   | 8    | 78   | 67   | 35   | 84   |
| <b>PBIAS</b> | Magoye      | 20   | 75   | 0    | 102  | 81   | 41   | 98   |
| <b>PBIAS</b> | Moorings    | 24   | 78   | 5    | 119  | 87   | 44   | 124  |
| <b>PBIAS</b> | Choma       | 9    | 60   | 0    | 102  | 65   | 20   | 99   |
| <b>PBIAS</b> | Livingstone | 29   | 54   | 8    | 89   | 87   | 33   | 86   |
| <b>PBIAS</b> | Petauke     | 15   | 61   | 17   | 70   | 66   | 45   | 75   |
| <b>PBIAS</b> | Mwinilunga  | 10   | 41   | 2    | 52   | 43   | 1    | 48   |
| <b>PBIAS</b> | Kasempa     | 3    | 46   | -2   | 50   | 39   | 2    | 50   |
| <b>PBIAS</b> | Kaoma       | 16   | 49   | 4    | 60   | 62   | 13   | 59   |
| <b>PBIAS</b> | Mongu       | 20   | 55   | 2    | 66   | 67   | 17   | 61   |
| <b>PBIAS</b> | Solwezi     | 13   | 58   | 8    | 55   | 52   | 12   | 61   |
| <b>PBIAS</b> | Zambezi     | 23   | 61   | 7    | 80   | 76   | 14   | 73   |
| <b>RSD</b>   | Chipata     | 1.02 | 1.2  | 1.15 | 1.35 | 1.22 | 1.02 | 1.23 |
| <b>RSD</b>   | Kasama      | 0.91 | 1.26 | 0.92 | 1.07 | 0.79 | 0.79 | 1.14 |
| <b>RSD</b>   | Mansa       | 0.84 | 0.78 | 0.78 | 0.71 | 0.67 | 0.73 | 0.67 |
| <b>RSD</b>   | Mpika       | 0.73 | 0.96 | 0.72 | 0.96 | 0.77 | 0.83 | 0.99 |

|            |             |       |       |       |       |       |       |       |
|------------|-------------|-------|-------|-------|-------|-------|-------|-------|
| <b>RSD</b> | Magoye      | 1.21  | 1.97  | 1.23  | 1.57  | 1.39  | 1.38  | 1.64  |
| <b>RSD</b> | Moorings    | 0.8   | 1.17  | 0.9   | 1.13  | 1.07  | 1.01  | 1.26  |
| <b>RSD</b> | Choma       | 1.35  | 1.36  | 1.22  | 1.34  | 1.59  | 1.35  | 1.47  |
| <b>RSD</b> | Livingstone | 1.21  | 1.53  | 1.24  | 1.55  | 1.59  | 1.33  | 1.64  |
| <b>RSD</b> | Petauke     | 1.17  | 1.67  | 1.31  | 1.34  | 1.34  | 1.18  | 1.35  |
| <b>RSD</b> | Mwinilunga  | 1.1   | 1.65  | 1.06  | 0.94  | 1.3   | 1.56  | 0.82  |
| <b>RSD</b> | Kasempa     | 0.82  | 1.22  | 1.03  | 0.85  | 1.1   | 0.88  | 0.8   |
| <b>RSD</b> | Kaoma       | 0.8   | 1.23  | 0.85  | 0.95  | 0.87  | 0.89  | 0.8   |
| <b>RSD</b> | Mongu       | 0.95  | 1.34  | 0.91  | 0.92  | 1.11  | 1.11  | 0.89  |
| <b>RSD</b> | Solwezi     | 0.83  | 1.29  | 0.83  | 0.85  | 0.94  | 0.81  | 0.78  |
| <b>RSD</b> | Zambezi     | 0.94  | 1.61  | 0.91  | 0.92  | 1.23  | 1.19  | 0.85  |
| <b>ME</b>  | Chipata     | 12.54 | 54.81 | 20.53 | 56.11 | 55.63 | 37.19 | 49.46 |
| <b>ME</b>  | Kasama      | -0.48 | 45.22 | 8.67  | 55.93 | 36.94 | 12.78 | 57    |
| <b>ME</b>  | Mansa       | 13.84 | 56.8  | 10.6  | 56.44 | 55.53 | 23.72 | 57.72 |
| <b>ME</b>  | Mpika       | 8.17  | 41.86 | 6.62  | 63.86 | 53.37 | 28.48 | 68.62 |
| <b>ME</b>  | Magoye      | 11.82 | 44.39 | -0.32 | 60.07 | 47.33 | 23.96 | 57.71 |
| <b>ME</b>  | Moorings    | 13.42 | 44.77 | 3     | 67.92 | 48.62 | 25.23 | 70.42 |

|    |             |       |       |       |       |       |       |       |
|----|-------------|-------|-------|-------|-------|-------|-------|-------|
| ME | Choma       | 5.67  | 39.89 | -0.19 | 67.78 | 42.18 | 13.48 | 65.33 |
| ME | Livingstone | 16.17 | 30.17 | 4.76  | 50    | 47.47 | 18.34 | 48.1  |
| ME | Petauke     | 10.94 | 43.03 | 12.21 | 49.91 | 46.52 | 31.73 | 53.15 |
| ME | Mwinilunga  | 11.41 | 47.86 | 1.76  | 59.5  | 48.42 | 0.64  | 55    |
| ME | Kasempa     | 2.71  | 43.43 | -1.5  | 47.43 | 36.42 | 2.14  | 47.14 |
| ME | Kaoma       | 11.96 | 37.46 | 3.32  | 45.96 | 46.31 | 9.96  | 45.35 |
| ME | Mongu       | 15.46 | 42.86 | 1.51  | 51.31 | 51.8  | 13.23 | 47.6  |
| ME | Solwezi     | 12.68 | 57.05 | 7.61  | 54.11 | 50.32 | 12.03 | 60    |
| ME | Zambezi     | 19.44 | 52.09 | 5.88  | 68.47 | 62.25 | 11.71 | 62.38 |

## Mean rain per rainy day – Zambia

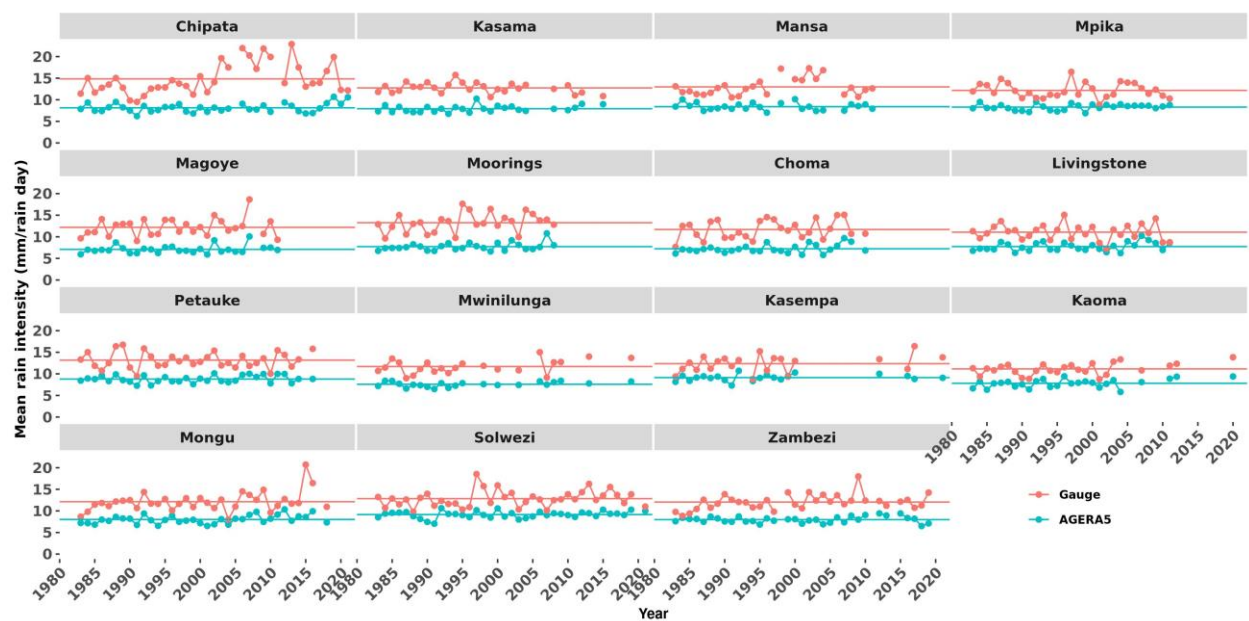

**Fig E45: Mean rain per rainy day across the stations in Zambia – rain gauge vs AGERA5. The horizontal lines represent average mean rain per rainy day across all the years considered for the gauge (red) and the AGERA5 (blue)**

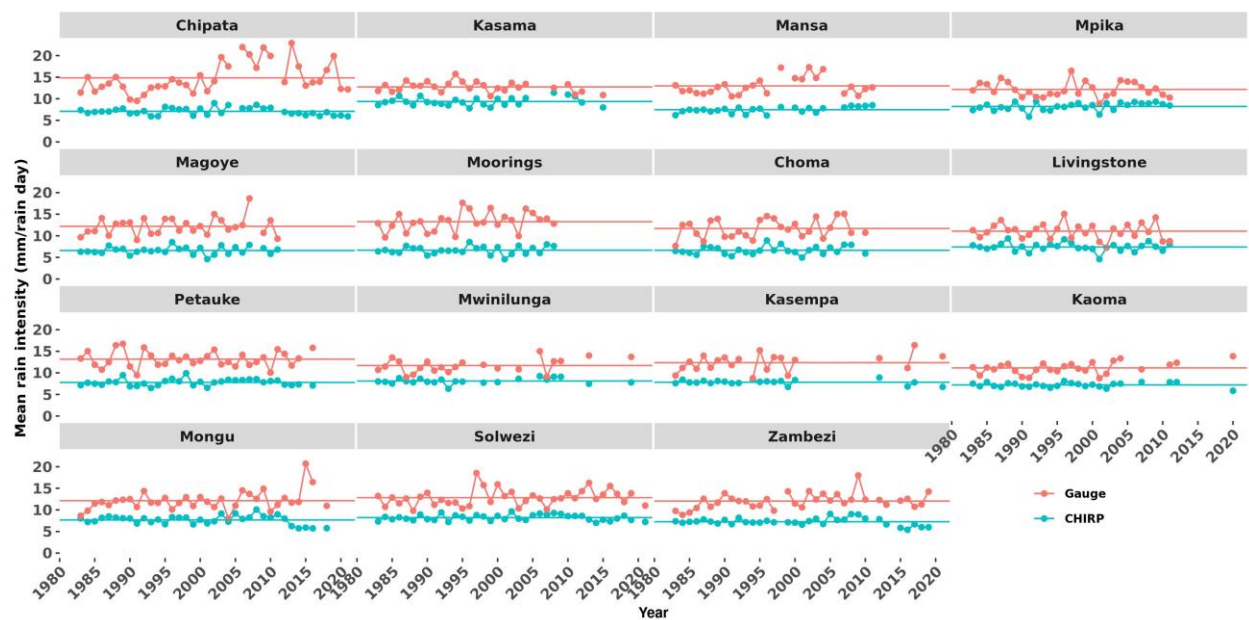

**Fig E46: Mean rain per rainy day across the stations in Zambia – rain gauge vs CHIRP. The horizontal lines represent average mean rain per rainy day across all the years considered for the gauge (red) and the CHIRP (blue)**

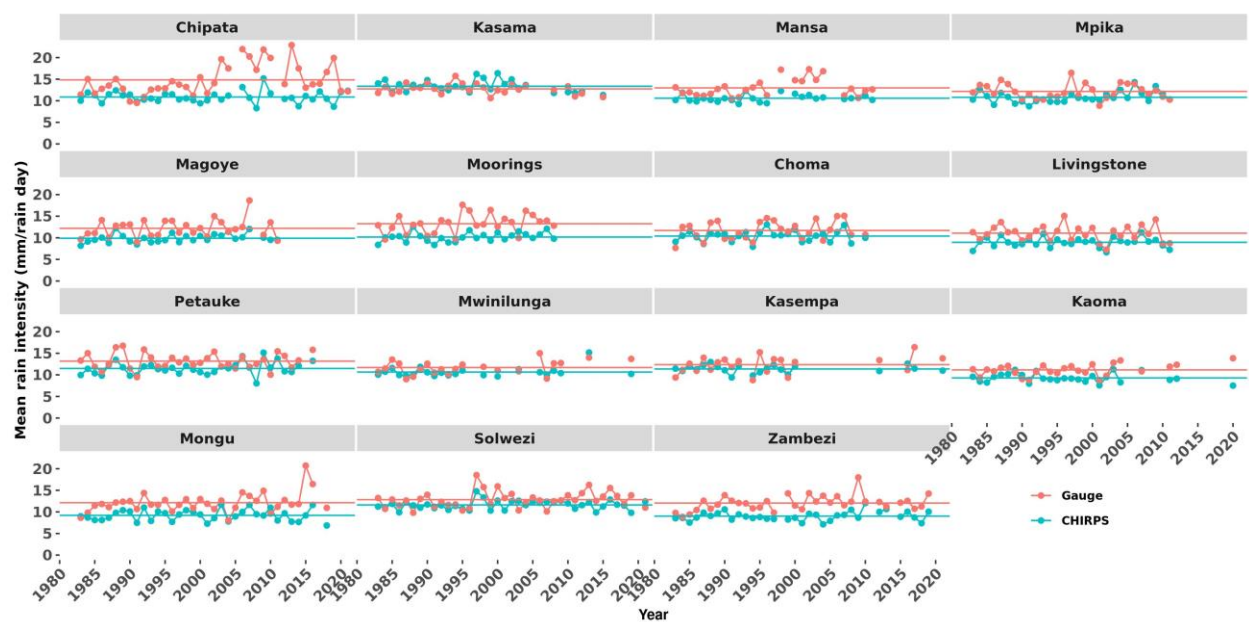

**Fig E47: Mean rain per rainy day across the stations in Zambia – rain gauge vs CHIRPS. The horizontal lines represent average mean rain per rainy day across all the years considered for the gauge (red) and the CHIRPS (blue)**

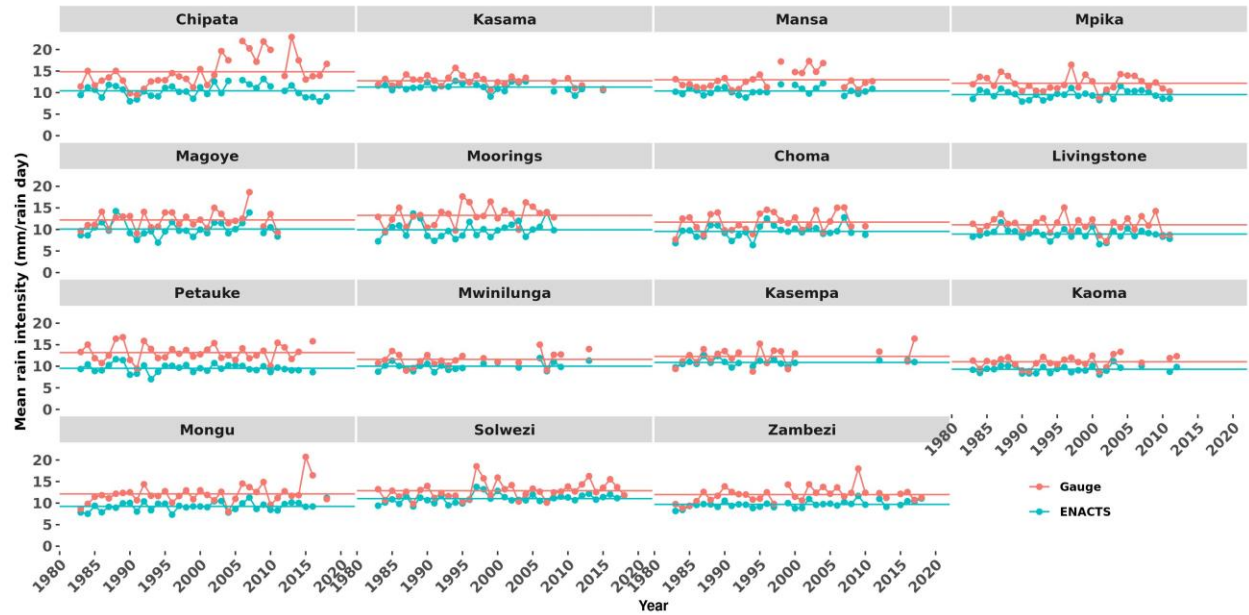

**Fig E48: Mean rain per rainy day across the stations in Zambia – rain gauge vs ENACTS.** The horizontal lines represent average mean rain per rainy day across all the years considered for the gauge (red) and the ENACTS (blue)

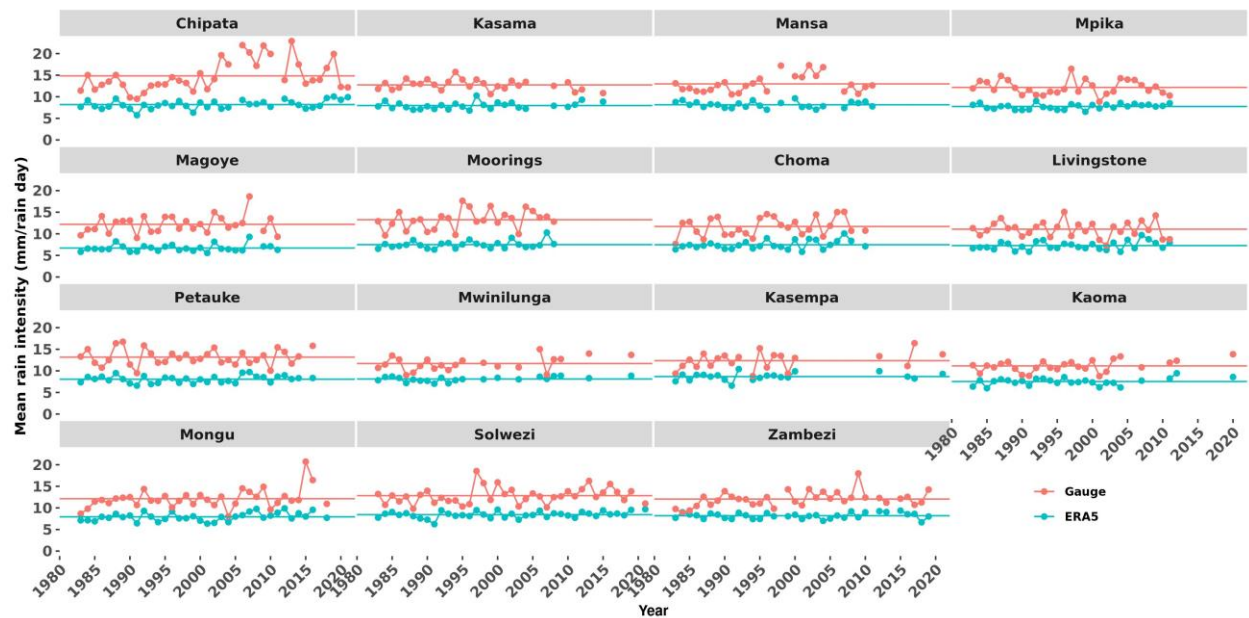

**Fig E49: Mean rain per rainy day across the stations in Zambia – rain gauge vs ERA5.** The horizontal lines represent average mean rain per rainy day across all the years considered for the gauge (red) and the ERA5 (blue)

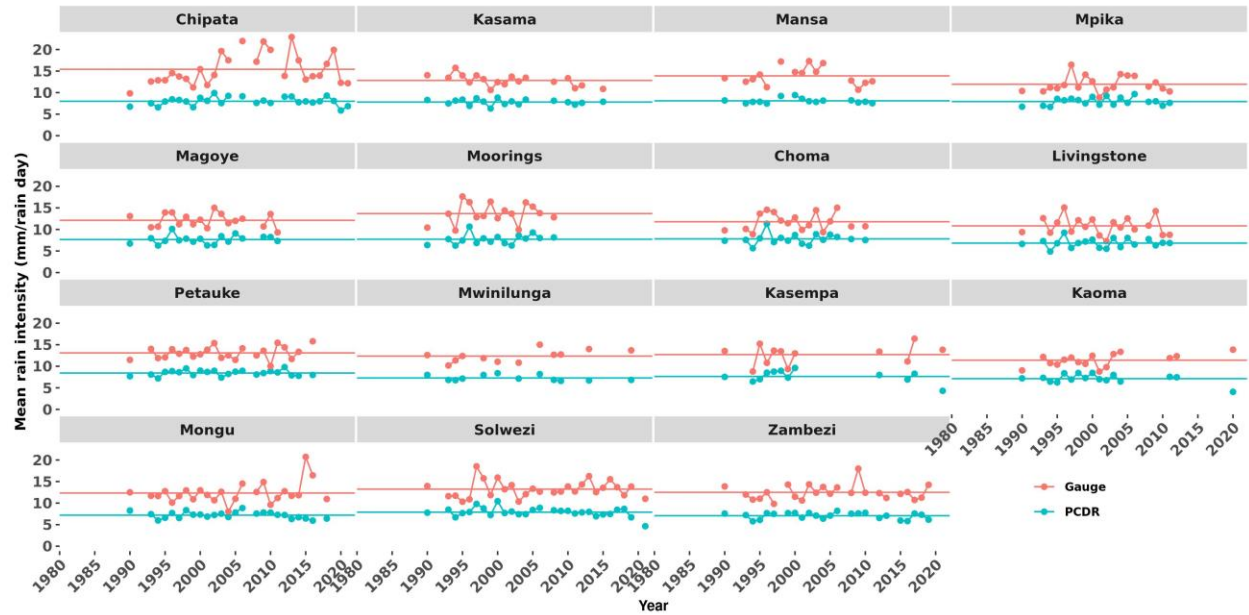

**Fig E50: Mean rain per rainy day across the stations in Zambia – rain gauge vs PCDR.** The horizontal lines represent the average mean rain per rainy day across all the years considered for the gauge (red) and the PCDR (blue)

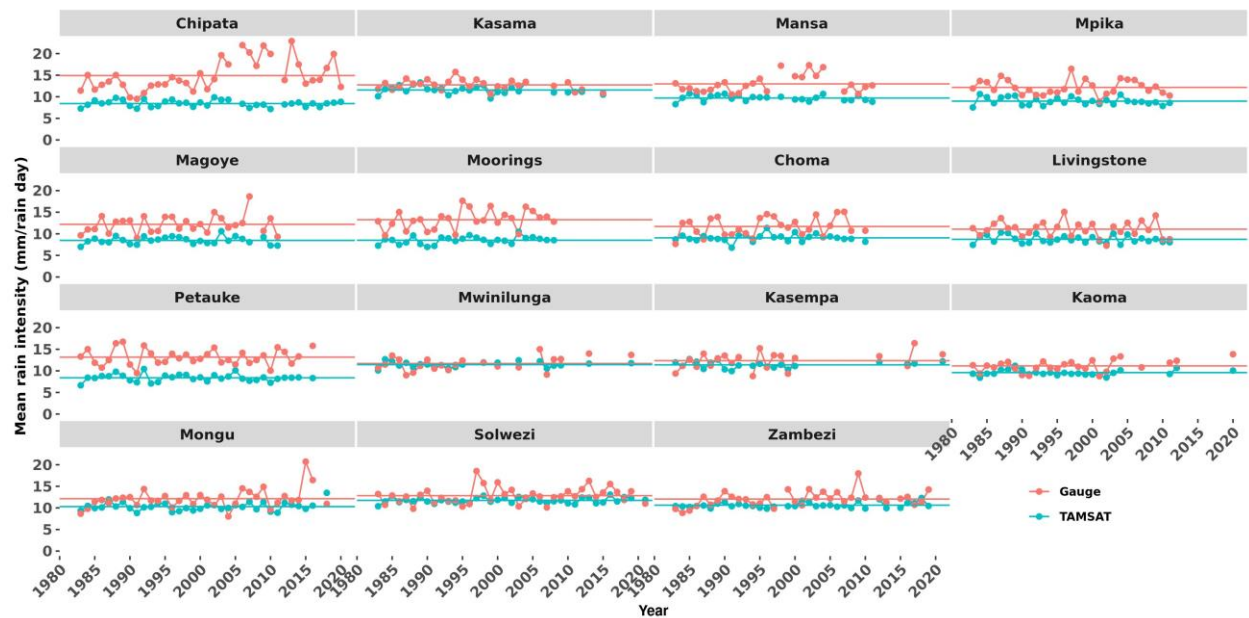

**Fig E51: Mean rain per rainy day across the stations in Zambia – rain gauge vs TAMSAT.** The horizontal lines represent the average mean rain per rainy day across all the years considered for the gauge (red) and the TAMSAT (blue)

**Table E3: Summary statistics on the performance of the products on mean rain per rainy day at the various stations in Zambia**

| metric | station     | CHIRPS | CHIRP | ENACTS | ERA5  | PCDR  | TAMSAT | AGERA5 |
|--------|-------------|--------|-------|--------|-------|-------|--------|--------|
| r      | Chipata     | 0.18   | 0.28  | 0.64   | 0.39  | 0.45  | 0.04   | 0.29   |
| r      | Kasama      | 0.36   | 0.26  | 0.66   | 0.04  | 0.59  | 0.37   | 0.07   |
| r      | Mansa       | 0.47   | 0.19  | 0.61   | 0     | 0.57  | -0.05  | 0.08   |
| r      | Mpika       | 0.49   | 0.27  | 0.77   | 0.17  | 0.47  | 0.55   | 0.21   |
| r      | Magoye      | 0.68   | 0.24  | 0.7    | 0.75  | 0.25  | 0.25   | 0.74   |
| r      | Moorings    | 0.23   | -0.12 | 0.11   | 0.16  | 0.34  | 0.13   | 0.07   |
| r      | Choma       | 0.7    | 0.47  | 0.84   | 0.62  | 0.65  | 0.43   | 0.53   |
| r      | Livingstone | 0.58   | 0.36  | 0.78   | 0.47  | 0.67  | 0.53   | 0.51   |
| r      | Petauke     | 0.44   | 0.19  | 0.53   | 0.49  | 0.31  | 0.37   | 0.47   |
| r      | Mwinilunga  | 0.46   | 0.24  | 0.82   | 0.65  | 0.05  | 0.43   | 0.67   |
| r      | Kasempa     | 0.22   | 0.17  | 0.6    | 0.23  | 0.13  | 0.11   | 0.15   |
| r      | Kaoma       | 0.07   | 0.22  | 0.67   | 0.29  | -0.17 | 0.32   | 0.37   |
| r      | Mongu       | 0.4    | -0.19 | 0.38   | 0.35  | -0.1  | 0.12   | 0.41   |
| r      | Solwezi     | 0.52   | 0.15  | 0.8    | 0.38  | 0.52  | 0.37   | 0.34   |
| r      | Zambezi     | 0.21   | 0.26  | 0.68   | -0.14 | 0.23  | 0.27   | -0.03  |

|              |             |      |      |      |      |      |      |      |
|--------------|-------------|------|------|------|------|------|------|------|
| <b>PBIAS</b> | Chipata     | -27  | -52  | -30  | -45  | -48  | -44  | -45  |
| <b>PBIAS</b> | Kasama      | 5    | -26  | -11  | -38  | -39  | -9   | -38  |
| <b>PBIAS</b> | Mansa       | -18  | -42  | -20  | -37  | -42  | -25  | -35  |
| <b>PBIAS</b> | Mpika       | -11  | -32  | -22  | -36  | -34  | -26  | -32  |
| <b>PBIAS</b> | Magoye      | -19  | -46  | -17  | -45  | -37  | -30  | -42  |
| <b>PBIAS</b> | Moorings    | -23  | -50  | -25  | -43  | -44  | -36  | -42  |
| <b>PBIAS</b> | Choma       | -11  | -43  | -18  | -36  | -34  | -22  | -38  |
| <b>PBIAS</b> | Livingstone | -19  | -33  | -19  | -34  | -37  | -21  | -30  |
| <b>PBIAS</b> | Petauke     | -13  | -41  | -28  | -39  | -36  | -36  | -33  |
| <b>PBIAS</b> | Mwinilunga  | -9   | -31  | -14  | -31  | -41  | -2   | -35  |
| <b>PBIAS</b> | Kasempa     | -8   | -37  | -11  | -30  | -40  | -8   | -26  |
| <b>PBIAS</b> | Kaoma       | -17  | -35  | -16  | -32  | -38  | -14  | -30  |
| <b>PBIAS</b> | Mongu       | -24  | -37  | -24  | -34  | -42  | -15  | -34  |
| <b>PBIAS</b> | Solwezi     | -10  | -36  | -14  | -34  | -40  | -9   | -29  |
| <b>PBIAS</b> | Zambezi     | -25  | -40  | -19  | -32  | -43  | -12  | -34  |
| <b>RSD</b>   | Chipata     | 0.37 | 0.23 | 0.41 | 0.28 | 0.26 | 0.2  | 0.28 |
| <b>RSD</b>   | Kasama      | 1.16 | 0.83 | 0.8  | 0.69 | 0.49 | 0.78 | 0.66 |

|            |             |       |       |       |       |       |       |       |
|------------|-------------|-------|-------|-------|-------|-------|-------|-------|
| <b>RSD</b> | Mansa       | 0.41  | 0.35  | 0.43  | 0.36  | 0.28  | 0.34  | 0.41  |
| <b>RSD</b> | Mpika       | 0.75  | 0.53  | 0.56  | 0.36  | 0.48  | 0.5   | 0.4   |
| <b>RSD</b> | Magoye      | 0.48  | 0.41  | 0.86  | 0.4   | 0.63  | 0.41  | 0.45  |
| <b>RSD</b> | Moorings    | 0.5   | 0.42  | 0.84  | 0.41  | 0.5   | 0.39  | 0.42  |
| <b>RSD</b> | Choma       | 0.6   | 0.45  | 0.7   | 0.47  | 0.63  | 0.41  | 0.46  |
| <b>RSD</b> | Livingstone | 0.62  | 0.54  | 0.61  | 0.53  | 0.51  | 0.47  | 0.55  |
| <b>RSD</b> | Petauke     | 0.81  | 0.42  | 0.53  | 0.45  | 0.45  | 0.46  | 0.46  |
| <b>RSD</b> | Mwinilunga  | 0.74  | 0.41  | 0.6   | 0.35  | 0.47  | 0.42  | 0.36  |
| <b>RSD</b> | Kasempa     | 0.46  | 0.28  | 0.39  | 0.44  | 0.62  | 0.39  | 0.4   |
| <b>RSD</b> | Kaoma       | 0.79  | 0.41  | 0.64  | 0.62  | 0.73  | 0.51  | 0.73  |
| <b>RSD</b> | Mongu       | 0.58  | 0.46  | 0.44  | 0.42  | 0.31  | 0.42  | 0.43  |
| <b>RSD</b> | Solwezi     | 0.56  | 0.37  | 0.54  | 0.4   | 0.55  | 0.33  | 0.42  |
| <b>RSD</b> | Zambezi     | 0.61  | 0.48  | 0.45  | 0.39  | 0.42  | 0.36  | 0.42  |
| <b>ME</b>  | Chipata     | -3.97 | -7.76 | -4.42 | -6.65 | -7.42 | -6.49 | -6.7  |
| <b>ME</b>  | Kasama      | 0.61  | -3.38 | -1.46 | -4.78 | -5.02 | -1.18 | -4.81 |
| <b>ME</b>  | Mansa       | -2.39 | -5.51 | -2.6  | -4.83 | -5.79 | -3.27 | -4.58 |
| <b>ME</b>  | Mpika       | -1.37 | -3.95 | -2.62 | -4.41 | -4.01 | -3.19 | -3.87 |

|           |             |       |       |       |       |       |       |       |
|-----------|-------------|-------|-------|-------|-------|-------|-------|-------|
| <b>ME</b> | Magoye      | -2.3  | -5.6  | -2.11 | -5.49 | -4.46 | -3.72 | -5.1  |
| <b>ME</b> | Moorings    | -3.08 | -6.59 | -3.34 | -5.76 | -5.95 | -4.75 | -5.53 |
| <b>ME</b> | Choma       | -1.29 | -5.05 | -2.15 | -4.24 | -3.97 | -2.64 | -4.48 |
| <b>ME</b> | Livingstone | -2.12 | -3.66 | -2.14 | -3.8  | -3.99 | -2.35 | -3.33 |
| <b>ME</b> | Petauke     | -1.7  | -5.4  | -3.66 | -5.12 | -4.67 | -4.8  | -4.39 |
| <b>ME</b> | Mwinilunga  | -1.05 | -3.58 | -1.59 | -3.58 | -5.08 | -0.25 | -4.11 |
| <b>ME</b> | Kasempa     | -1    | -4.53 | -1.4  | -3.68 | -5.07 | -0.97 | -3.22 |
| <b>ME</b> | Kaoma       | -1.87 | -3.95 | -1.73 | -3.63 | -4.29 | -1.55 | -3.33 |
| <b>ME</b> | Mongu       | -2.92 | -4.46 | -2.89 | -4.19 | -5.13 | -1.83 | -4.11 |
| <b>ME</b> | Solwezi     | -1.23 | -4.63 | -1.83 | -4.41 | -5.34 | -1.1  | -3.69 |
| <b>ME</b> | Zambezi     | -3.02 | -4.78 | -2.27 | -3.86 | -5.42 | -1.42 | -4.06 |

## Annual Total Rainfall – Ghana

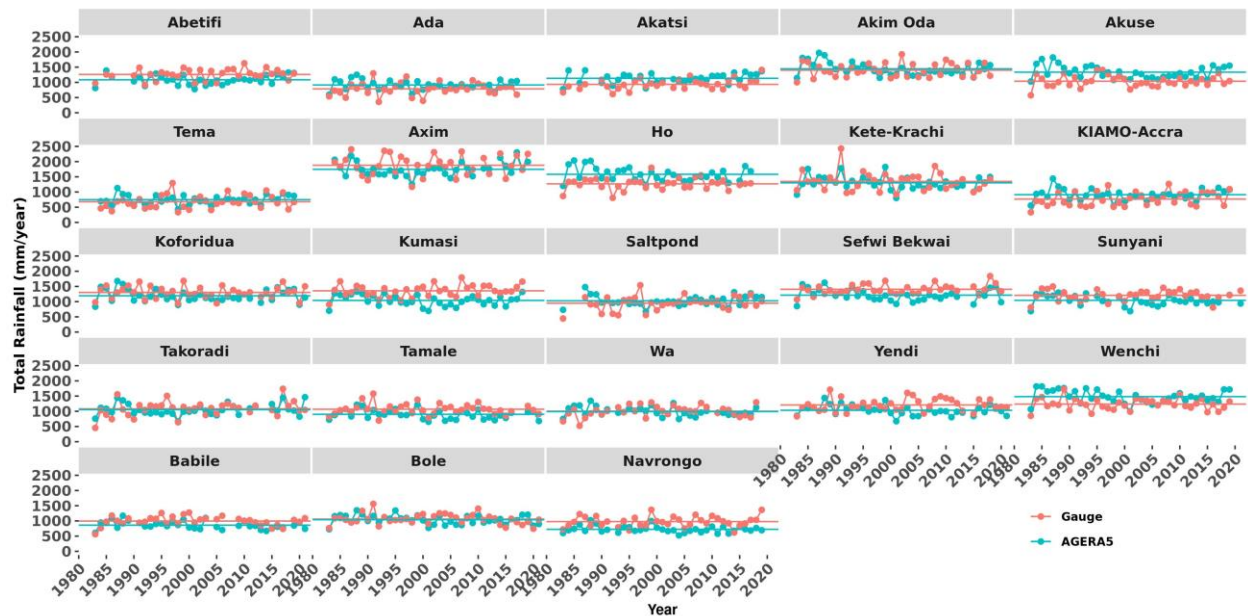

**Fig E52: Total annual rainfall across the stations in Ghana – rain gauge vs AGERA5.** The horizontal lines represent mean annual total rainfall across all the years considered for the gauge (red) and the AGERA5 (blue).

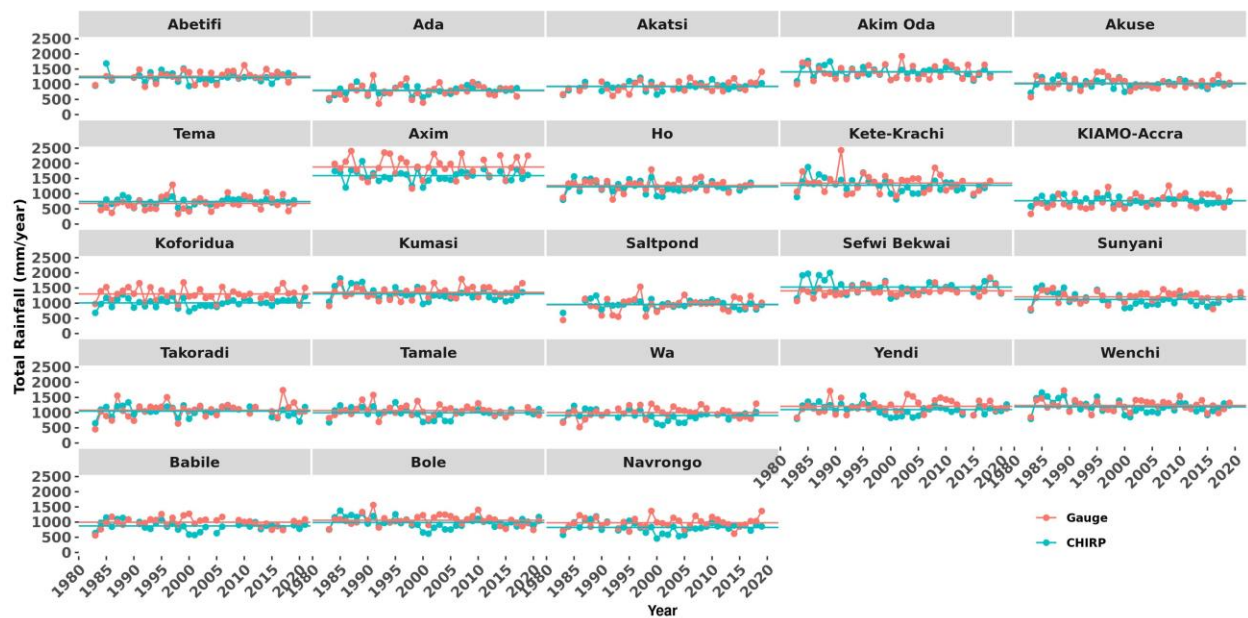

**Fig E53: Total annual rainfall across the stations in Ghana – rain gauge vs CHIRP.** The horizontal lines represent mean annual total rainfall across all the years considered for the gauge (red) and the CHIRP (blue).

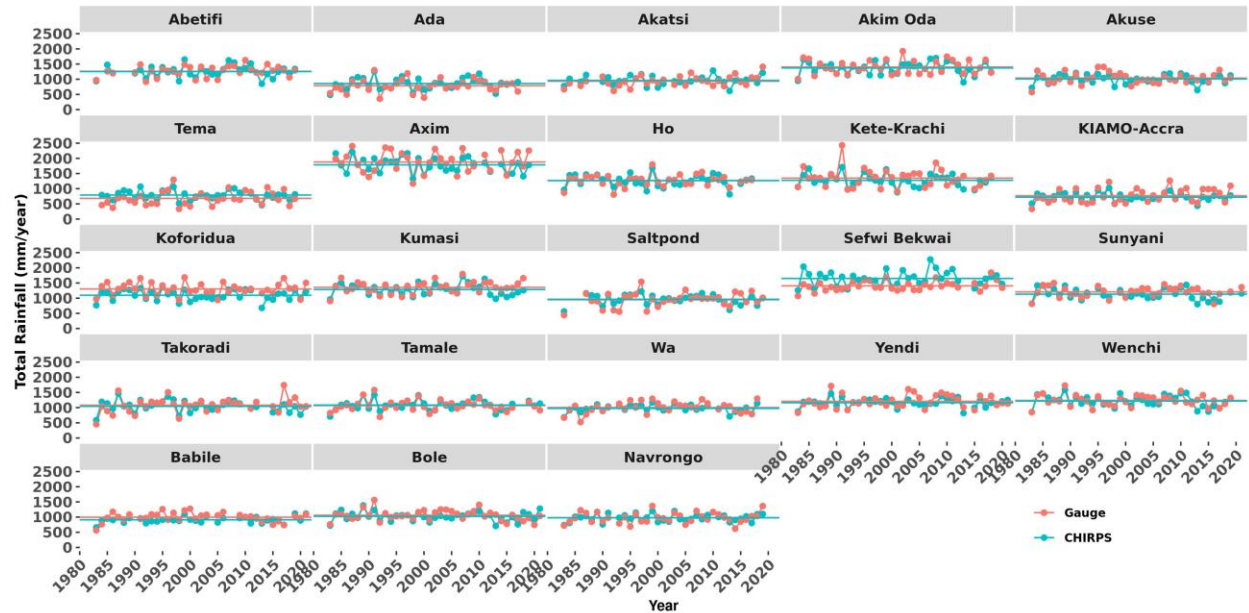

**Fig E54: Total annual rainfall across the stations in Ghana – rain gauge vs CHIRPS.** The horizontal lines represent mean annual total rainfall across all the years considered for the gauge (red) and the CHIRPS (blue).

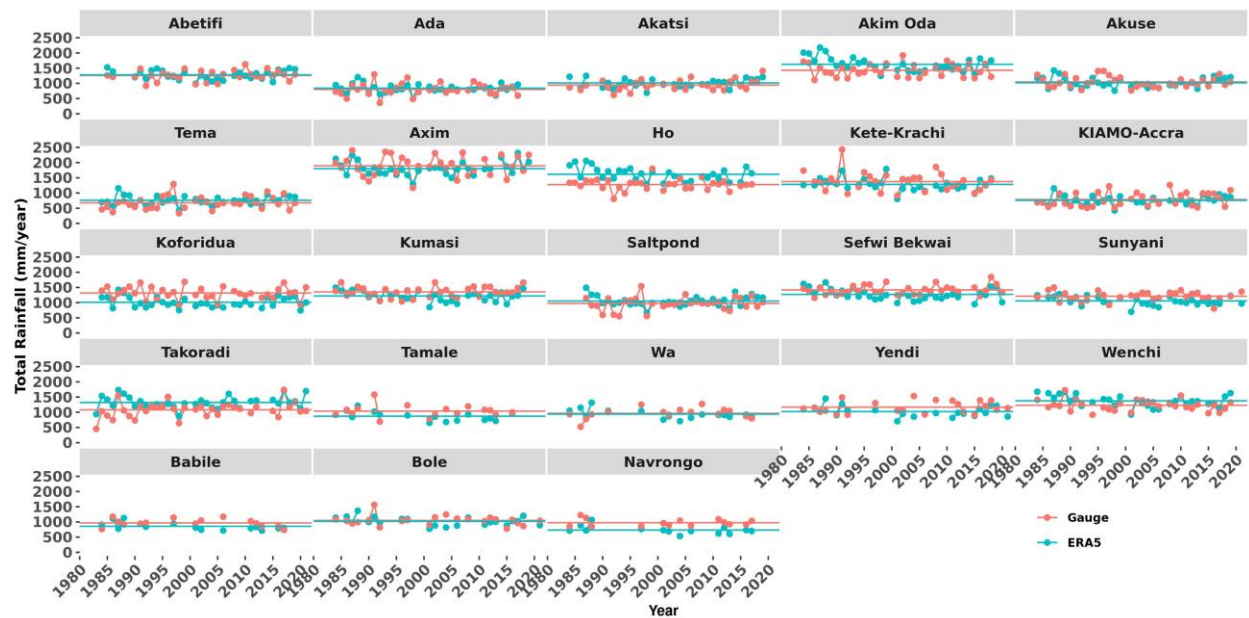

**Fig E55: Total annual rainfall across the stations in Ghana – rain gauge vs ERA5.** The horizontal lines represent mean annual total rainfall across all the years considered for the gauge (red) and the ERA5 (blue).

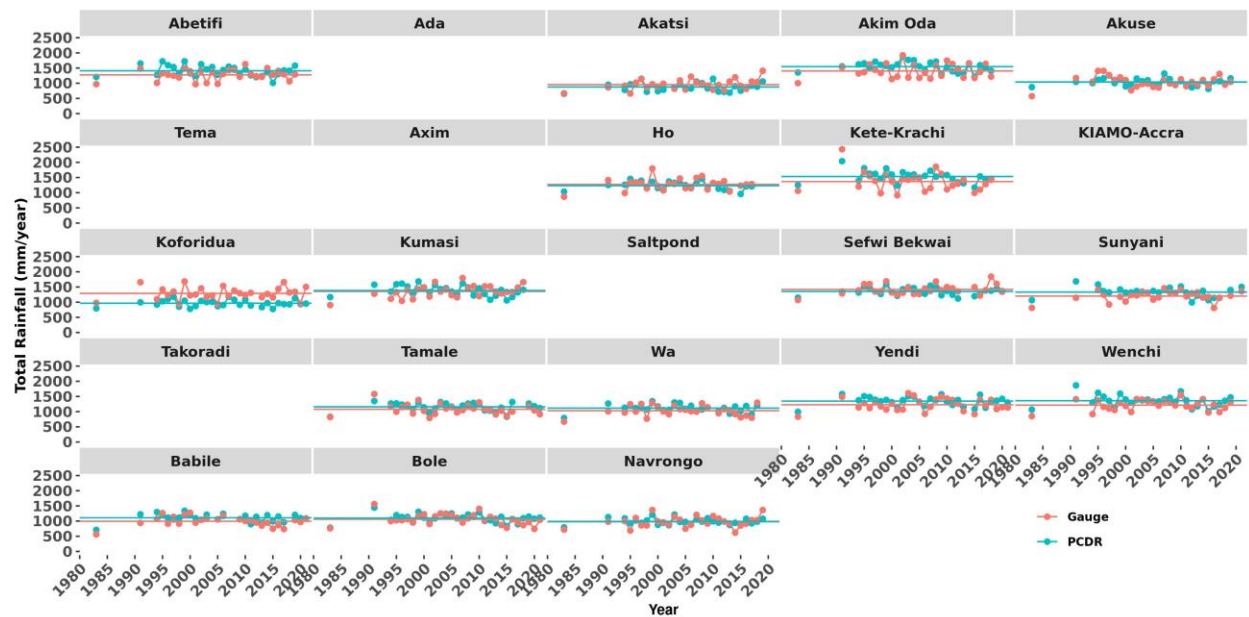

**Fig E56: Total annual rainfall across the stations in Ghana – rain gauge vs PCDR. The horizontal lines represent mean annual total rainfall across all the years considered for the gauge (red) and the PCDR (blue).**

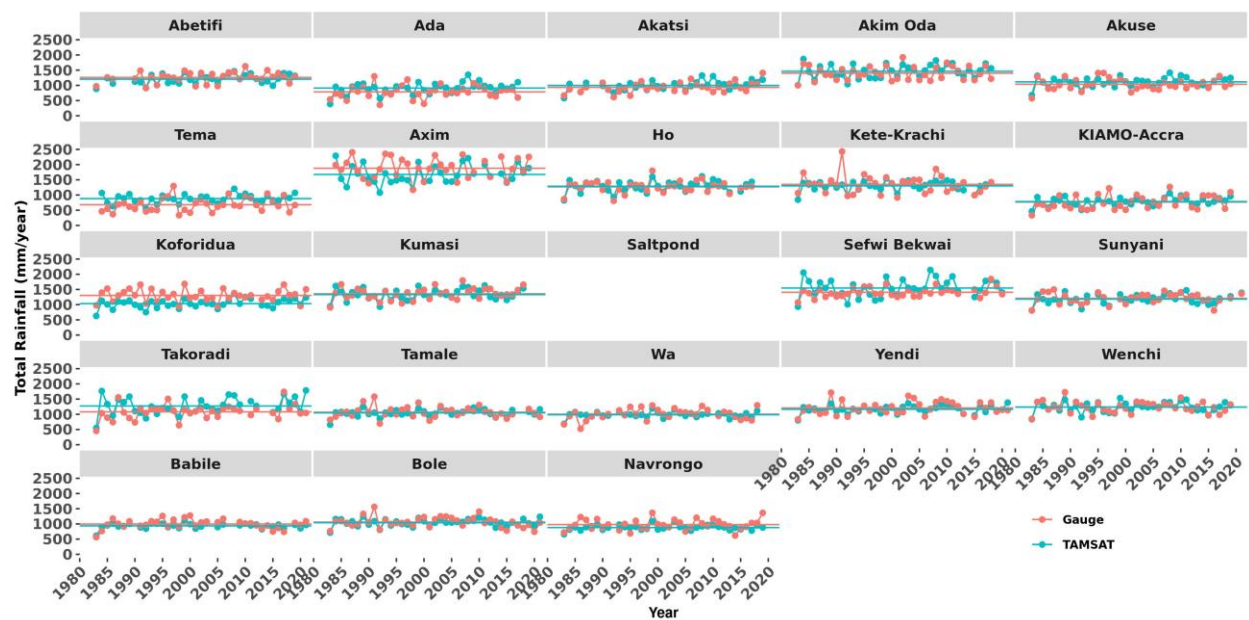

**Fig E57: Total annual rainfall across the stations in Ghana – rain gauge vs TAMSAT. The horizontal lines represent mean annual total rainfall across all the years considered for the gauge (red) and the TAMSAT (blue).**

**Table E4: Summary statistics on the performance of the products on annual total rainfall at the various stations in Ghana**

| <b>metric</b> | <b>station</b> | <b>CHIRPS</b> | <b>CHIRP</b> | <b>ERA5</b> | <b>TAMSA T</b> | <b>AGERAS</b> | <b>PCDR</b> |
|---------------|----------------|---------------|--------------|-------------|----------------|---------------|-------------|
| <b>r</b>      | Abetifi        | 0.56          | 0.42         | 0.23        | 0.55           | 0.33          | 0.48        |
| <b>r</b>      | Ada            | 0.72          | 0.62         | 0.43        | 0.5            | 0.43          | NA          |
| <b>r</b>      | Akatsi         | 0.19          | 0.22         | 0.21        | 0.35           | 0.31          | 0.35        |
| <b>r</b>      | Akim Oda       | 0.59          | 0.64         | 0.28        | 0.59           | 0.36          | 0.38        |
| <b>r</b>      | Akuse          | 0.49          | 0.5          | 0.31        | 0.5            | 0.38          | 0.55        |
| <b>r</b>      | Tema           | 0.68          | 0.66         | 0.39        | 0.39           | 0.41          | NA          |
| <b>r</b>      | Axim           | 0.53          | 0.29         | 0.45        | 0.33           | 0.46          | NA          |
| <b>r</b>      | Ho             | 0.7           | 0.64         | 0.42        | 0.74           | 0.46          | 0.61        |
| <b>r</b>      | Kete-Krachi    | 0.59          | 0.33         | 0.51        | 0.45           | 0.44          | 0.7         |
| <b>r</b>      | KIAMO-Accra    | 0.72          | 0.42         | 0.27        | 0.56           | 0.36          | NA          |
| <b>r</b>      | Koforidua      | 0.65          | 0.65         | 0.45        | 0.6            | 0.52          | 0.36        |
| <b>r</b>      | Kumasi         | 0.63          | 0.36         | 0.46        | 0.66           | 0.45          | 0.2         |
| <b>r</b>      | Saltpond       | 0.69          | 0.44         | 0.3         | NA             | 0.36          | NA          |
| <b>r</b>      | Sefwi Bekwai   | 0.45          | 0.45         | 0.22        | 0.49           | 0.35          | 0.49        |
| <b>r</b>      | Sunyani        | 0.53          | 0.48         | 0.16        | 0.49           | 0.31          | 0.42        |

|              |             |      |      |       |      |      |      |
|--------------|-------------|------|------|-------|------|------|------|
| <b>r</b>     | Takoradi    | 0.69 | 0.49 | 0.57  | 0.51 | 0.52 | NA   |
| <b>r</b>     | Tamale      | 0.81 | 0.36 | 0.38  | 0.58 | 0.56 | 0.75 |
| <b>r</b>     | Wa          | 0.69 | 0.13 | -0.24 | 0.56 | 0.25 | 0.63 |
| <b>r</b>     | Yendi       | 0.7  | 0.2  | 0.11  | 0.73 | 0.18 | 0.68 |
| <b>r</b>     | Wenchi      | 0.69 | 0.56 | 0.47  | 0.59 | 0.51 | 0.69 |
| <b>r</b>     | Babile      | 0.5  |      | 0.14  | 0.74 | 0.33 | 0.68 |
| <b>r</b>     | Bole        | 0.56 | 0.23 | 0.13  | 0.59 | 0.35 | 0.73 |
| <b>r</b>     | Navrongo    | 0.64 | 0.2  | -0.11 | 0.42 | 0.29 | 0.58 |
| <b>PBIAS</b> | Abetifi     | 0    | -3   | 2     | -4   | -14  | 11   |
| <b>PBIAS</b> | Ada         | 9    | 2    | 5     | 16   | 16   | NA   |
| <b>PBIAS</b> | Akatsi      | 3    | -1   | 7     | 7    | 21   | -8   |
| <b>PBIAS</b> | Akim Oda    | -2   | 1    | 14    | 4    | 3    | 10   |
| <b>PBIAS</b> | Akuse       | -3   | -2   | -2    | 8    | 29   | 0    |
| <b>PBIAS</b> | Tema        | 16   | 9    | 12    | 29   | 10   | NA   |
| <b>PBIAS</b> | Axim        | -5   | -15  | -5    | -11  | -7   | NA   |
| <b>PBIAS</b> | Ho          | 0    | -3   | 27    | 2    | 25   | -3   |
| <b>PBIAS</b> | Kete-Krachi | -5   | -5   | -7    | -3   | -3   | 12   |

|              |              |      |      |      |      |      |      |
|--------------|--------------|------|------|------|------|------|------|
| <b>PBIAS</b> | KIAMO-Accra  | -6   | 0    | -3   | 2    | 19   | NA   |
| <b>PBIAS</b> | Koforidua    | -16  | -23  | -23  | -21  | -8   | -25  |
| <b>PBIAS</b> | Kumasi       | -5   | -4   | -10  | -2   | -23  | 2    |
| <b>PBIAS</b> | Saltpond     | 1    | 1    | 8    | NA   | 8    | NA   |
| <b>PBIAS</b> | Sefwi Bekwai | 17   | 9    | -10  | 10   | -14  | -5   |
| <b>PBIAS</b> | Sunyani      | -6   | -7   | -13  | -2   | -14  | 11   |
| <b>PBIAS</b> | Takoradi     | -4   | -3   | 22   | 18   | -2   | NA   |
| <b>PBIAS</b> | Tamale       | 2    | -7   | -16  | -2   | -16  | 8    |
| <b>PBIAS</b> | Wa           | -3   | -10  | -3   | -2   | -1   | 8    |
| <b>PBIAS</b> | Yendi        | -4   | -9   | -13  | -3   | -14  | 10   |
| <b>PBIAS</b> | Wenchi       | -2   | -4   | 12   | 0    | 20   | 12   |
| <b>PBIA</b>  | Babile       | -8   | -12  | -12  | -6   | -14  | 11   |
| <b>PBIAS</b> | Bole         | -3   | -7   | -3   | -2   | -2   | 4    |
| <b>PBIAS</b> | Navrongo     | 0    | -16  | -25  | -10  | -26  | 1    |
| <b>RSD</b>   | Abetifi      | 1.1  | 0.95 | 0.89 | 0.9  | 0.89 | 0.98 |
| <b>RSD</b>   | Ada          | 0.89 | 0.67 | 0.73 | 0.88 | 0.72 | NA   |
| <b>RSD</b>   | Akatsi       | 0.84 | 0.77 | 0.82 | 0.91 | 0.95 | 0.82 |

|            |              |      |      |      |      |      |      |
|------------|--------------|------|------|------|------|------|------|
| <b>RSD</b> | Akim Oda     | 0.91 | 0.77 | 1.04 | 0.98 | 0.93 | 0.71 |
| <b>RSD</b> | Akuse        | 0.81 | 0.75 | 0.96 | 0.85 | 1.13 | 0.67 |
| <b>RSD</b> | Tema         | 0.65 | 0.47 | 0.68 | 0.63 | 0.64 | NA   |
| <b>RSD</b> | Axim         | 0.73 | 0.57 | 0.68 | 0.92 | 0.68 | NA   |
| <b>RSD</b> | Ho           | 1    | 0.97 | 1.17 | 0.96 | 1.15 | 0.69 |
| <b>RSD</b> | Kete-Krachi  | 0.67 | 0.75 | 0.64 | 0.53 | 0.73 | 0.6  |
| <b>RSD</b> | KIAMO-Accra  | 0.58 | 0.5  | 0.66 | 0.59 | 0.76 | NA   |
| <b>RSD</b> | Koforidua    | 0.86 | 0.71 | 0.84 | 0.73 | 0.99 | 0.55 |
| <b>RSD</b> | Kumasi       | 0.94 | 1.01 | 0.99 | 0.95 | 0.9  | 0.83 |
| <b>RSD</b> | Saltpond     | 0.7  | 0.58 | 0.77 | NA   | 0.72 | NA   |
| <b>RSD</b> | Sefwi Bekwai | 1.49 | 1.4  | 1.2  | 1.83 | 1.19 | 0.72 |
| <b>RSD</b> | Sunyani      | 1.04 | 1.19 | 0.93 | 0.93 | 0.94 | 0.96 |
| <b>RSD</b> | Takoradi     | 0.76 | 0.67 | 0.8  | 1.13 | 0.77 | NA   |
| <b>RSD</b> | Tamale       | 0.94 | 0.91 | 0.75 | 0.66 | 0.86 | 0.8  |
| <b>RSD</b> | Wa           | 0.64 | 0.86 | 0.84 | 0.52 | 0.83 | 0.74 |
| <b>RSD</b> | Yendi        | 0.67 | 0.83 | 0.87 | 0.59 | 0.77 | 0.76 |
| <b>RSD</b> | Wenchi       | 1.03 | 1.14 | 1.06 | 0.89 | 1.15 | 1.08 |

|            |                 |         |         |         |         |         |        |
|------------|-----------------|---------|---------|---------|---------|---------|--------|
| <b>RSD</b> | Babile          | 0.66    | 0.97    | 0.96    | 0.58    | 0.85    | 0.82   |
| <b>RSD</b> | Bole            | 0.87    | 1.02    | 0.91    | 0.7     | 0.87    | 0.78   |
| <b>RSD</b> | Navrongo        | 0.72    | 0.95    | 1.11    | 0.47    | 0.63    | 0.57   |
| <b>ME</b>  | Abetifi         | -6.91   | -40.98  | 20.07   | -56.28  | -175.06 | 135.6  |
| <b>ME</b>  | Ada             | 73.22   | 17.94   | 39.35   | 125.61  | 128.61  | NA     |
| <b>ME</b>  | Akatsi          | 25.94   | -9.45   | 69.56   | 62.25   | 198.13  | -77.63 |
| <b>ME</b>  | Akim Oda        | -29.97  | 9.5     | 197.41  | 62.56   | 43.63   | 143.13 |
| <b>ME</b>  | Akuse           | -26.71  | -21.85  | -26.41  | 77.85   | 298.13  | -5.26  |
| <b>ME</b>  | Tema            | 109.81  | 61.11   | 81.54   | 199.7   | 66.31   | NA     |
| <b>ME</b>  | Axim            | -94.16  | -284.36 | -91.44  | -204.05 | -132.47 | NA     |
| <b>ME</b>  | Ho              | -0.71   | -43.34  | 339.62  | 18.88   | 314.52  | -43.12 |
| <b>ME</b>  | Kete-Krachi     | -72.12  | -70.05  | -92.85  | -46.5   | -45.78  | 166.34 |
| <b>ME</b>  | KIAMO-<br>Accra | -45.35  | 3.25    | -26.55  | 17.31   | 144.97  | NA     |
| <b>ME</b>  | Koforidua       | -207.35 | -294.15 | -306.13 | -268.84 | -109.33 | -324.5 |
| <b>ME</b>  | Kumasi          | -70.78  | -50.3   | -132.35 | -23.89  | -316.51 | 28.91  |
| <b>ME</b>  | Saltpond        | 13.29   | 11.11   | 80.31   | NA      | 79.05   | NA     |

|           |                 |        |         |         |        |         |        |
|-----------|-----------------|--------|---------|---------|--------|---------|--------|
| <b>ME</b> | Sefwi<br>Bekwai | 243.11 | 124.19  | -146.83 | 141.76 | -192.8  | -66.61 |
| <b>ME</b> | Sunyani         | -75.75 | -84.97  | -152.54 | -25.62 | -163.91 | 131    |
| <b>ME</b> | Takoradi        | -37.97 | -31.43  | 240.56  | 192.69 | -25.28  | NA     |
| <b>ME</b> | Tamale          | 16.68  | -73.23  | -166.96 | -20.11 | -167.38 | 80.94  |
| <b>ME</b> | Wa              | -27.8  | -96.67  | -26.56  | -17.43 | -11.25  | 85.39  |
| <b>ME</b> | Yendi           | -45.33 | -105.35 | -147.18 | -41.36 | -173.97 | 118.9  |
| <b>ME</b> | Wenchi          | -19.54 | -46.13  | 145.33  | 0.01   | 245.55  | 145.63 |
| <b>ME</b> | Babile          | -84.9  | -123.07 | -110.7  | -59.71 | -135.34 | 112.86 |
| <b>ME</b> | Bole            | -36.45 | -71.93  | -28.68  | -17.91 | -18.14  | 38.91  |
| <b>ME</b> | Navrongo        | 1.63   | -153.04 | -241.48 | -97.45 | -254.11 | 11.02  |

## Annual Number of Rainy Days – Ghana

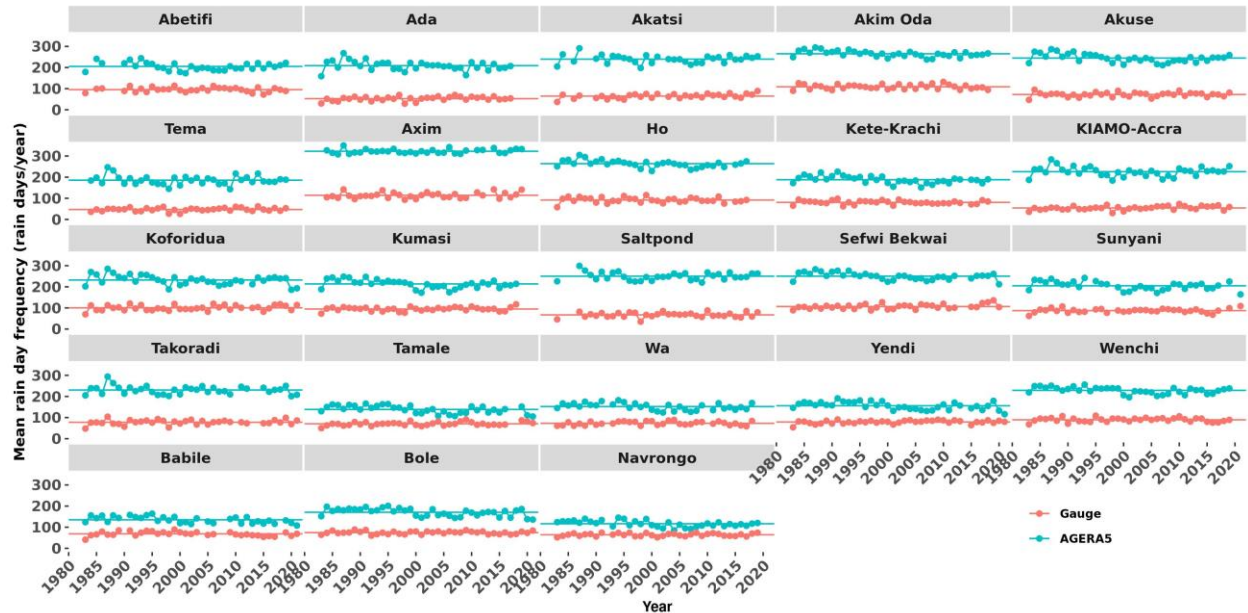

**Fig E58: Annual number of rainy days across the stations in Ghana – rain gauge vs AGERA5. The horizontal lines represent mean number of rainy days across all the years considered for the gauge (red) and the AGERA5 (blue).**

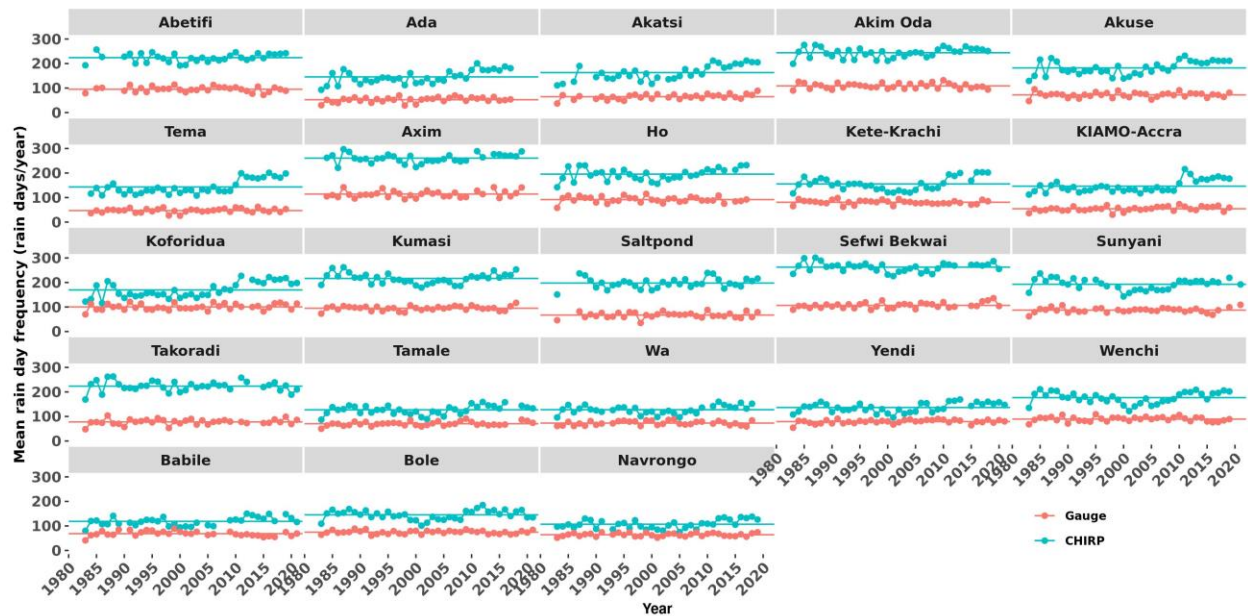

**Fig E59: Annual number of rainy days across the stations in Ghana – rain gauge vs CHIRP. The horizontal lines represent mean number of rainy days across all the years considered for the gauge (red) and the CHIRP (blue).**

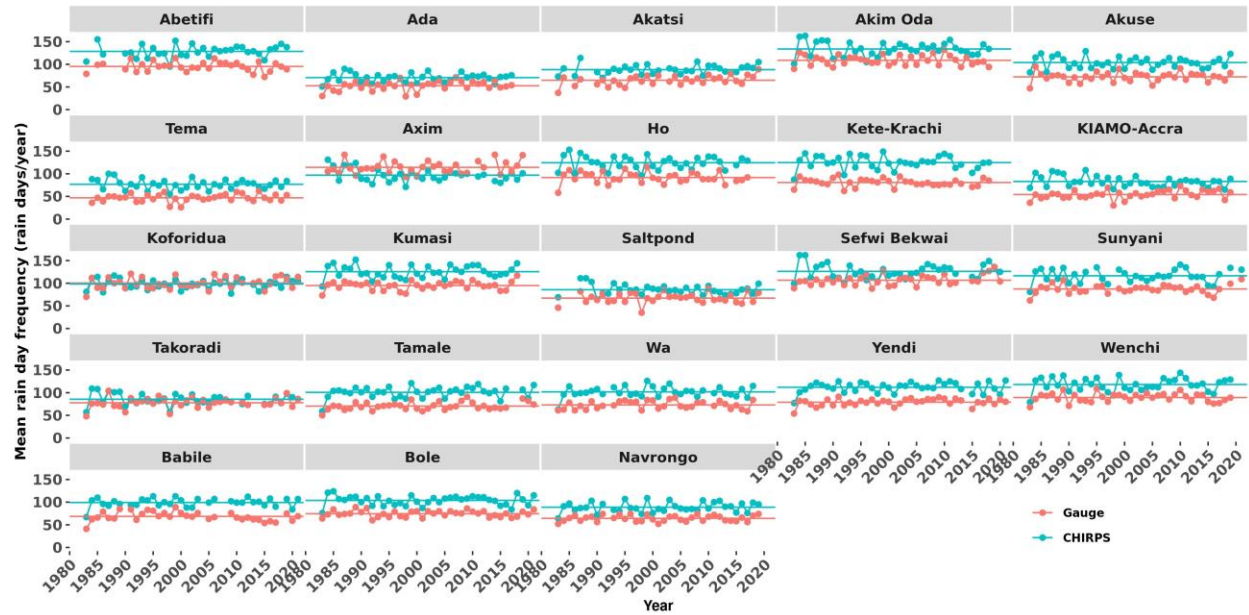

**Fig E60: Annual number of rainy days across the stations in Ghana – rain gauge vs CHIRPS. The horizontal lines represent mean number of rainy days across all the years considered for the gauge (red) and the CHIRPS (blue).**

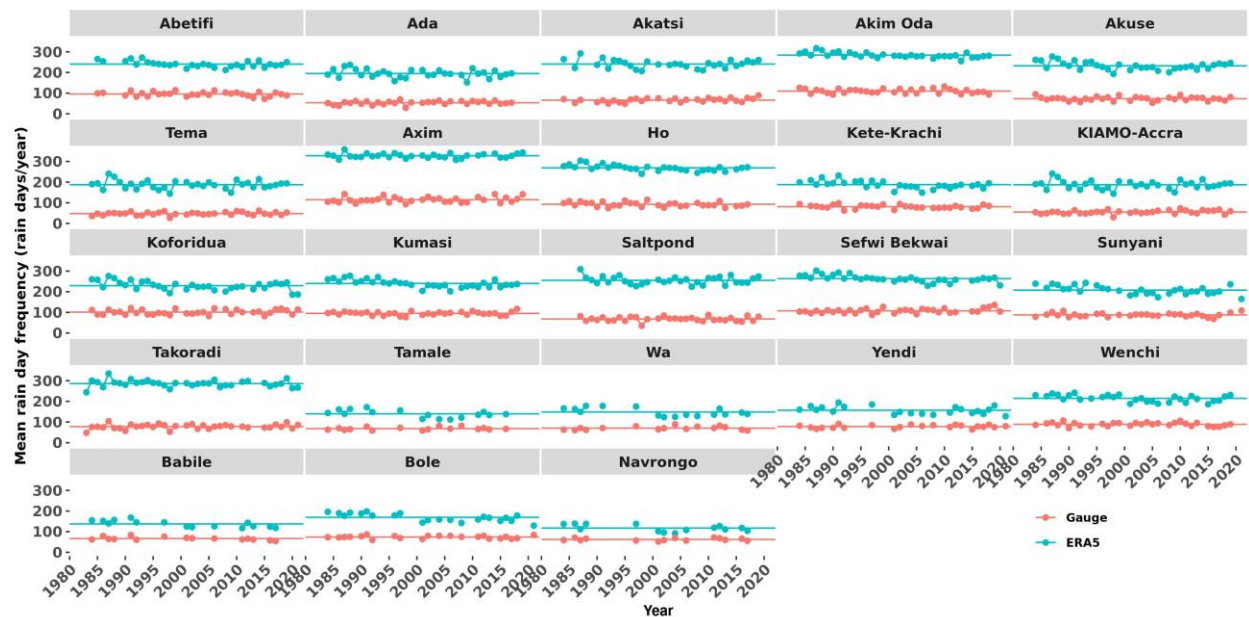

**Fig E61: Annual number of rainy days across the stations in Ghana – rain gauge vs ERA5. The horizontal lines represent mean number of rainy days across all the years considered for the gauge (red) and the ERA5 (blue).**

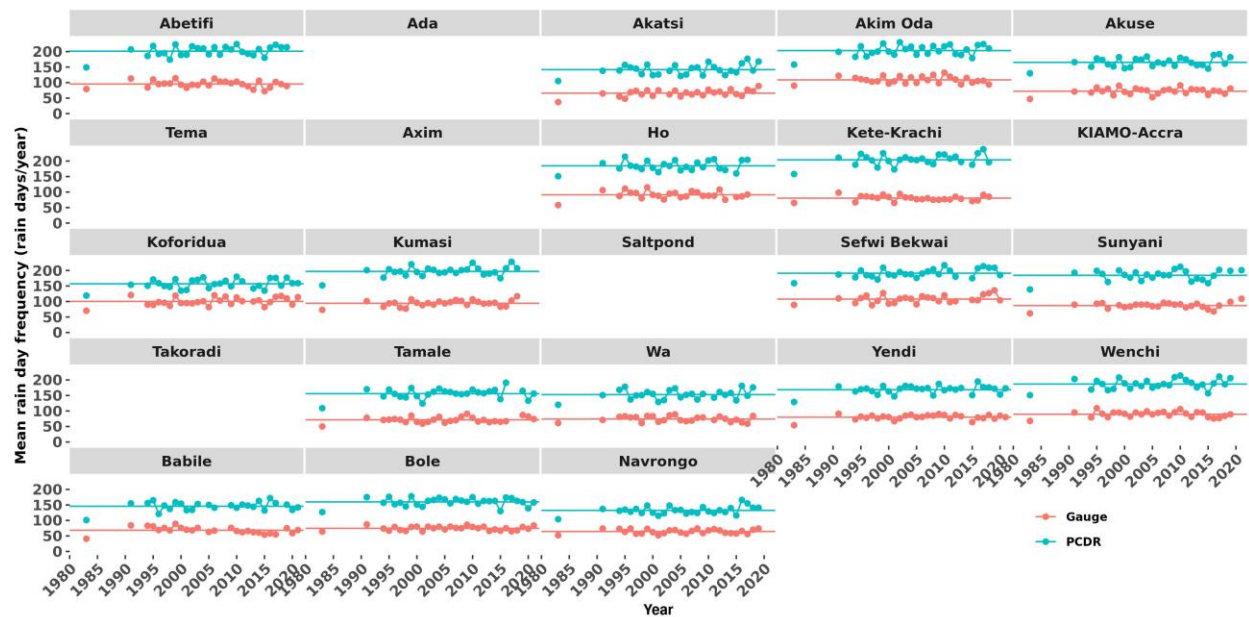

**Fig E62: Annual number of rainy days across the stations in Ghana – rain gauge vs PCDR. The horizontal lines represent mean number of rainy days across all the years considered for the gauge (red) and the PCDR (blue).**

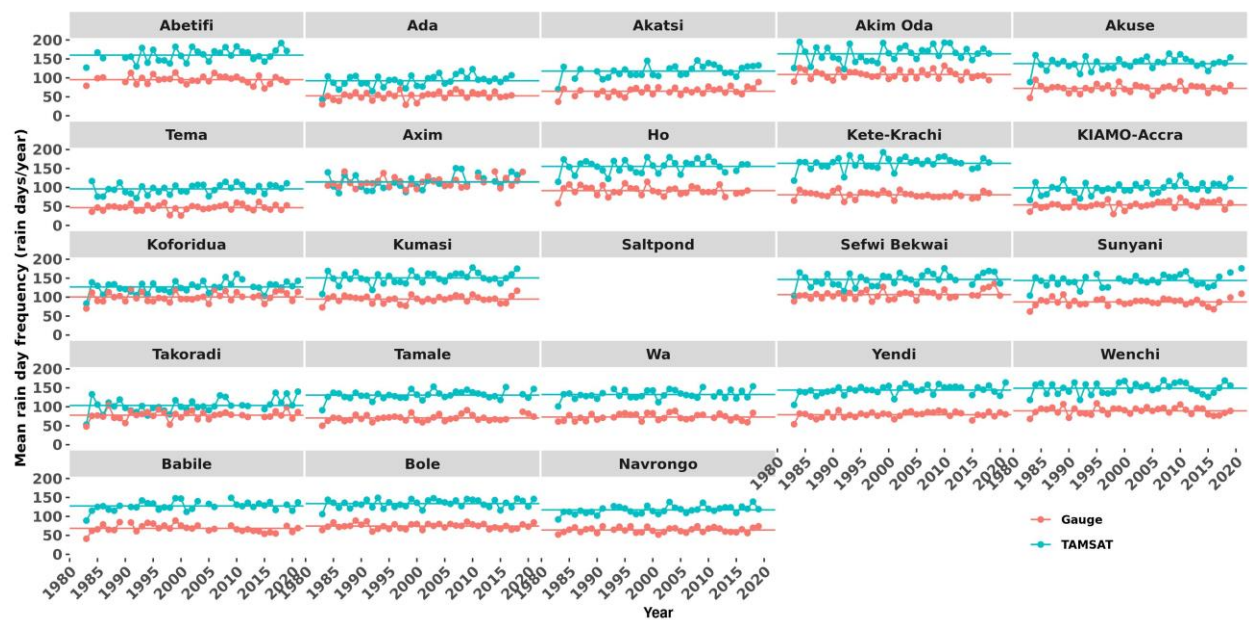

**Fig E63: Annual number of rainy days across the stations in Ghana – rain gauge vs TAMSAT. The horizontal lines represent mean number of rainy days across all the years considered for the gauge (red) and the TAMSAT (blue).**

**Table E5: Summary statistics on the performance of the products on annual number of rainy days at the various stations in Ghana**

| <b>metric</b> | <b>station</b> | <b>CHIRPS</b> | <b>CHIRP</b> | <b>ERA5</b> | <b>TAMSAT</b> | <b>AGERA5</b> | <b>PCDR</b> |
|---------------|----------------|---------------|--------------|-------------|---------------|---------------|-------------|
| <b>r</b>      | Abetifi        | 0.47          | 0.49         | 0.23        | 0.56          | 0.25          | 0.61        |
| <b>r</b>      | Ada            | 0.45          | 0.45         | 0.35        | 0.73          | 0.4           | NA          |
| <b>r</b>      | Akatsi         | 0.53          | 0.51         | 0.32        | 0.59          | 0.49          | 0.57        |
| <b>r</b>      | Akim Oda       | 0.59          | 0.46         | 0.31        | 0.6           | 0.3           | 0.57        |
| <b>r</b>      | Akuse          | 0.64          | 0.32         | 0.35        | 0.72          | 0.33          | 0.67        |
| <b>r</b>      | Tema           | 0.35          | 0.33         | 0.42        | 0.3           | 0.44          | NA          |
| <b>r</b>      | Axim           | 0.08          | 0.49         | 0.57        | 0.26          | 0.51          | NA          |
| <b>r</b>      | Ho             | 0.6           | 0.44         | 0.45        | 0.58          | 0.38          | 0.53        |
| <b>r</b>      | Kete-Krachi    | 0.57          | 0.14         | 0.38        | 0.64          | 0.35          | 0.58        |
| <b>r</b>      | KIAMO-Accra    | 0.25          | 0.43         | 0.32        | 0.45          | 0.36          | NA          |
| <b>r</b>      | Koforidua      | 0.47          | 0.39         | 0.23        | 0.63          | 0.35          | 0.55        |
| <b>r</b>      | Kumasi         | 0.71          | 0.41         | 0.16        | 0.79          | 0.2           | 0.68        |
| <b>r</b>      | Saltpond       | 0.37          | 0.54         | 0.31        | NA            | 0.41          | NA          |
| <b>r</b>      | Sefwi Bekwai   | 0.39          | 0.33         | 0           | 0.71          | 0.15          | 0.73        |
| <b>r</b>      | Sunyani        | 0.67          | 0.24         | 0.06        | 0.62          | 0.14          | 0.62        |
| <b>r</b>      | Takoradi       | 0.53          | 0.5          | 0.62        | 0.51          | 0.5           | NA          |

|              |             |      |       |       |      |      |      |
|--------------|-------------|------|-------|-------|------|------|------|
| <b>r</b>     | Tamale      | 0.6  | 0.29  | -0.02 | 0.62 | 0.06 | 0.44 |
| <b>r</b>     | Wa          | 0.57 | 0.19  | -0.17 | 0.52 | 0.15 | 0.47 |
| <b>r</b>     | Yendi       | 0.59 | 0.24  | 0.22  | 0.73 | 0.08 | 0.64 |
| <b>r</b>     | Wenchi      | 0.63 | 0.21  | 0.07  | 0.54 | 0.13 | 0.53 |
| <b>r</b>     | Babile      | 0.52 | -0.02 | 0.57  | 0.59 | 0.53 | 0.49 |
| <b>r</b>     | Bole        | 0.52 | 0.23  | 0.03  | 0.47 | 0.08 | 0.37 |
| <b>r</b>     | Navrongo    | 0.48 | 0.13  | 0.29  | 0.43 | 0.24 | 0.31 |
| <b>PBIAS</b> | Abetifi     | 35   | 135   | 152   | 68   | 115  | 111  |
| <b>PBIAS</b> | Ada         | 34   | 177   | 265   | 76   | 297  | NA   |
| <b>PBIAS</b> | Akatsi      | 36   | 152   | 264   | 82   | 270  | 115  |
| <b>PBIAS</b> | Akim Oda    | 23   | 124   | 159   | 50   | 144  | 87   |
| <b>PBIAS</b> | Akuse       | 44   | 152   | 218   | 90   | 239  | 129  |
| <b>PBIAS</b> | Tema        | 64   | 205   | 295   | 105  | 296  | NA   |
| <b>PBIAS</b> | Axim        | -15  | 128   | 186   | 1    | 182  | NA   |
| <b>PBIAS</b> | Ho          | 36   | 113   | 191   | 70   | 187  | 102  |
| <b>PBIAS</b> | Kete-Krachi | 54   | 92    | 132   | 103  | 133  | 154  |
| <b>PBIAS</b> | KIAMO-Accra | 53   | 170   | 240   | 83   | 317  | NA   |

|              |              |      |      |      |      |      |      |
|--------------|--------------|------|------|------|------|------|------|
| <b>PBIAS</b> | Koforidua    | -2   | 69   | 126  | 26   | 131  | 56   |
| <b>PBIAS</b> | Kumasi       | 32   | 128  | 152  | 59   | 125  | 109  |
| <b>PBIAS</b> | Saltpond     | 28   | 194  | 275  | NA   | 272  | NA   |
| <b>PBIAS</b> | Sefwi Bekwai | 18   | 146  | 145  | 38   | 135  | 77   |
| <b>PBIAS</b> | Sunyani      | 33   | 121  | 137  | 65   | 135  | 112  |
| <b>PBIAS</b> | Takorad      | 1    | 188  | 267  | 3    | 196  | NA   |
| <b>PBIAS</b> | Tamale       | 43   | 80   | 105  | 86   | 96   | 118  |
| <b>PBIAS</b> | Wa           | 40   | 75   | 111  | 82   | 10   | 10   |
| <b>PBIAS</b> | Yendi        | 42   | 73   | 101  | 82   | 97   | 111  |
| <b>PBIAS</b> | Wenchi       | 32   | 9    | 141  | 67   | 156  | 109  |
| <b>PBIAS</b> | Babile       | 45   | 73   | 106  | 86   | 97   | 114  |
| <b>PBIAS</b> | Bole         | 39   | 95   | 129  | 80   | 129  | 114  |
| <b>PBIAS</b> | Navrongo     | 38   | 67   | 88   | 82   | 81   | 106  |
| <b>RSD</b>   | Abetifi      | 1.26 | 1.62 | 1.37 | 1.57 | 1.71 | 1.57 |
| <b>RSD</b>   | Ada          | 0.92 | 2.6  | 2.33 | 1.58 | 2.14 | NA   |
| <b>RSD</b>   | Akatsi       | 0.96 | 2.85 | 2.06 | 1.5  | 1.79 | 1.58 |
| <b>RSD</b>   | Akim Oda     | 1.38 | 1.81 | 1.16 | 1.82 | 1.26 | 1.55 |

|            |              |      |      |      |      |      |      |
|------------|--------------|------|------|------|------|------|------|
| <b>RSD</b> | Akuse        | 1.18 | 2.66 | 1.97 | 1.51 | 1.88 | 1.48 |
| <b>RSD</b> | Tema         | 1.29 | 3.47 | 2.66 | 1.51 | 2.57 | NA   |
| <b>RSD</b> | Axim         | 1.02 | 1.31 | 0.8  | 1.34 | 0.73 | NA   |
| <b>RSD</b> | Ho           | 1.18 | 1.95 | 1.3  | 1.37 | 1.32 | 1.29 |
| <b>RSD</b> | Kete-Krachi  | 1.69 | 3.03 | 2.11 | 1.83 | 1.99 | 2.09 |
| <b>RSD</b> | KIAMO-Accra  | 1.24 | 2.66 | 2.36 | 1.57 | 2.33 | NA   |
| <b>RSD</b> | Koforidua    | 0.89 | 2.5  | 1.85 | 1.23 | 1.84 | 1.18 |
| <b>RSD</b> | Kumasi       | 1.45 | 2.3  | 2.11 | 1.61 | 2.12 | 1.56 |
| <b>RSD</b> | Saltpond     | 0.98 | 1.83 | 1.71 | NA   | 1.59 | NA   |
| <b>RSD</b> | Sefwi Bekwai | 1.4  | 1.6  | 1.5  | 1.48 | 1.46 | 1.14 |
| <b>RSD</b> | Sunyani      | 1.46 | 2.25 | 2.26 | 1.55 | 2.01 | 1.76 |
| <b>RSD</b> | Takoradi     | 1.08 | 1.82 | 1.43 | 1.62 | 1.7  | NA   |
| <b>RSD</b> | Tamale       | 1.41 | 2.08 | 2.56 | 1.33 | 2.09 | 1.79 |
| <b>RSD</b> | Wa           | 1.32 | 1.91 | 2.27 | 1.31 | 1.84 | 1.76 |
| <b>RSD</b> | Yendi        | 1.44 | 2.43 | 2.43 | 1.54 | 2.29 | 1.68 |
| <b>RSD</b> | Wenchi       | 1.5  | 2.41 | 1.82 | 1.52 | 1.58 | 1.73 |
| <b>RSD</b> | Babile       | 0.93 | 1.71 | 2.04 | 1.18 | 1.53 | 1.38 |

|            |              |        |        |        |       |        |        |
|------------|--------------|--------|--------|--------|-------|--------|--------|
| <b>RSD</b> | Bole         | 1.51   | 2.67   | 2.75   | 1.5   | 2.57   | 1.96   |
| <b>RSD</b> | Navrongo     | 1.61   | 2.65   | 2.6    | 1.5   | 2.17   | 1.8    |
| <b>ME</b>  | Abetifi      | 33.27  | 128.82 | 144.97 | 64.67 | 109.88 | 105.75 |
| <b>ME</b>  | Ada          | 18.06  | 93.03  | 141.66 | 39.77 | 156.31 | NA     |
| <b>ME</b>  | Akatsi       | 23.48  | 98.39  | 174.73 | 53.09 | 174.88 | 75.81  |
| <b>ME</b>  | Akim Oda     | 24.94  | 135.25 | 174.3  | 54.58 | 156.33 | 94.37  |
| <b>ME</b>  | Akuse        | 31.59  | 109.95 | 159.29 | 65.2  | 172.57 | 93.0   |
| <b>ME</b>  | Tema         | 29.97  | 96.28  | 139.88 | 49.42 | 138.83 | NA     |
| <b>ME</b>  | Axim         | -17.29 | 146.41 | 213.09 | 0.85  | 208.38 | NA     |
| <b>ME</b>  | Ho           | 32.62  | 103.68 | 176.52 | 63.94 | 171.97 | 93.4   |
| <b>ME</b>  | Kete-Krachi  | 44     | 74.66  | 106.67 | 83.09 | 107.2  | 123.46 |
| <b>ME</b>  | KIAMO-Accra  | 28.81  | 92.16  | 132.12 | 44.89 | 171.76 | NA     |
| <b>ME</b>  | Koforidua    | -2.18  | 69.13  | 128.03 | 26.53 | 131.68 | 56.72  |
| <b>ME</b>  | Kumasi       | 30.67  | 121.58 | 144.9  | 55.86 | 118.75 | 102.74 |
| <b>ME</b>  | Saltpond     | 18.56  | 130.44 | 187.12 | NA    | 183    | NA     |
| <b>ME</b>  | Sefwi Bekwai | 19.58  | 155.92 | 155.82 | 40.03 | 143.58 | 83.41  |
| <b>ME</b>  | Sunyani      | 29.14  | 105.37 | 120.1  | 56.57 | 117.6  | 97.5   |

|    |          |       |        |        |       |        |       |
|----|----------|-------|--------|--------|-------|--------|-------|
| ME | Takoradi | 7.72  | 145.86 | 208.34 | 25.75 | 152.44 | NA    |
| ME | Tamale   | 30.3  | 56.51  | 71.5   | 60.24 | 68     | 84.32 |
| ME | Wa       | 28.85 | 54.59  | 78.12  | 59.41 | 79.24  | 78.69 |
| ME | Yendi    | 32.97 | 57.71  | 78.95  | 64.97 | 76.92  | 88.52 |
| ME | Wenchi   | 28.81 | 87.54  | 125.73 | 59.57 | 139.41 | 97.32 |
| ME | Babile   | 30.71 | 49.97  | 70.93  | 59    | 66.68  | 77.54 |
| ME | Bole     | 29.36 | 70.67  | 95.23  | 59.36 | 96.13  | 85.27 |
| ME | Navrongo | 24.69 | 42.72  | 55     | 52.97 | 52.19  | 68.14 |

## Mean Rain Per Rainy Day – Ghana

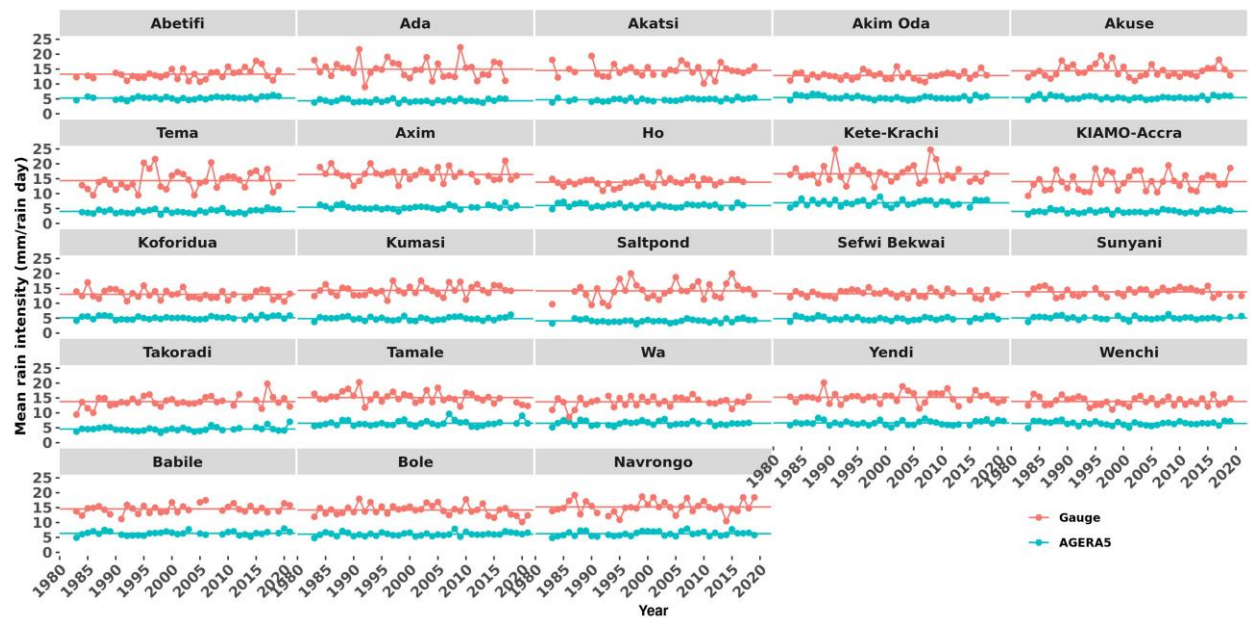

**Fig E64: Mean rain per rainy day across the stations in Ghana – rain gauge vs AGERA5. The horizontal lines represent the average mean rain per rainy day across all the years considered for the gauge (red) and the AGERA5 (blue)**

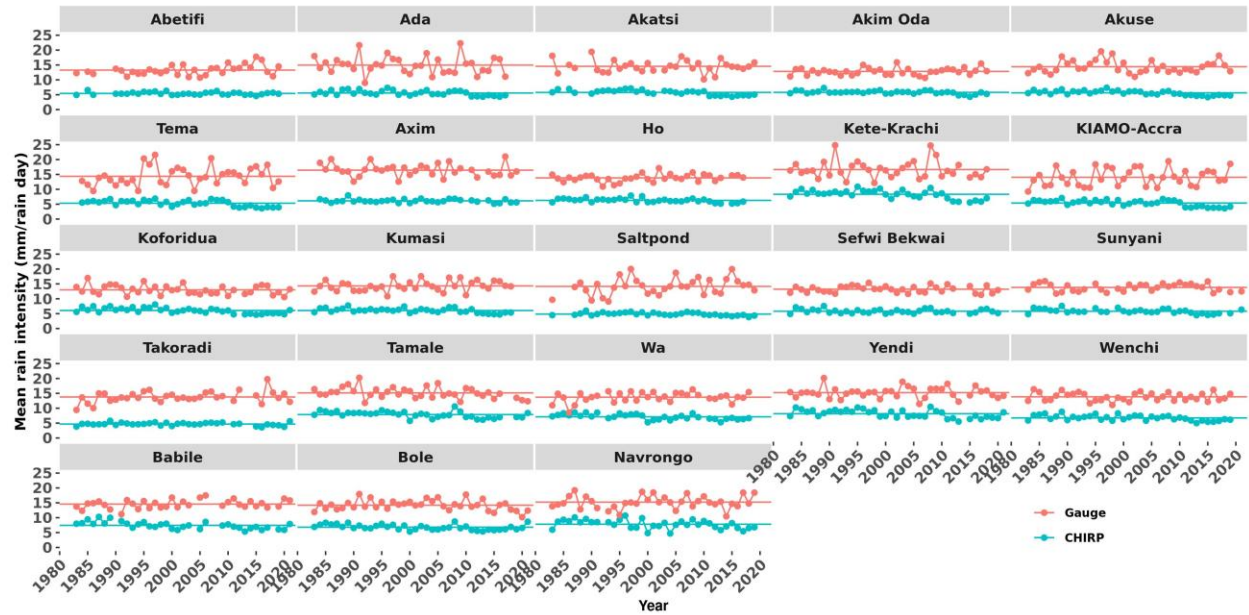

**Fig E65: Mean rain per rainy day across the stations in Ghana – rain gauge vs CHIRP. The horizontal lines represent the average mean rain per rainy day across all the years considered for the gauge (red) and the CHIRP (blue)**

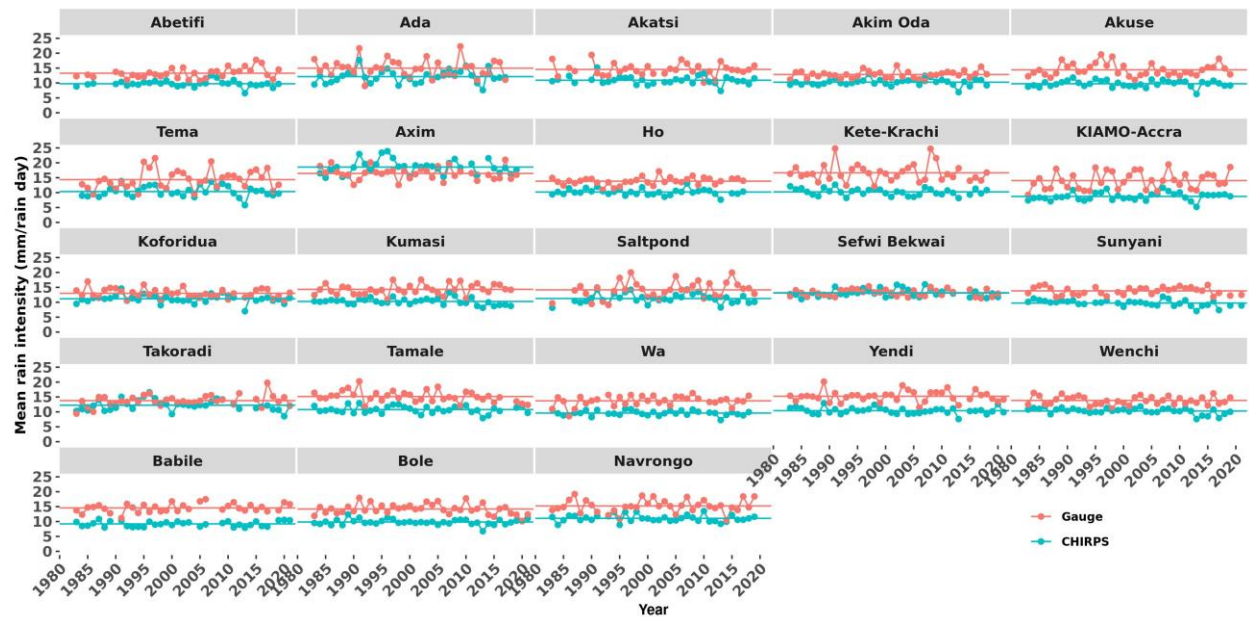

**Fig E66: Mean rain per rainy day across the stations in Ghana – rain gauge vs CHIRPS. The horizontal lines represent the average mean rain per rainy day across all the years considered for the gauge (red) and the CHIRPS (blue)**

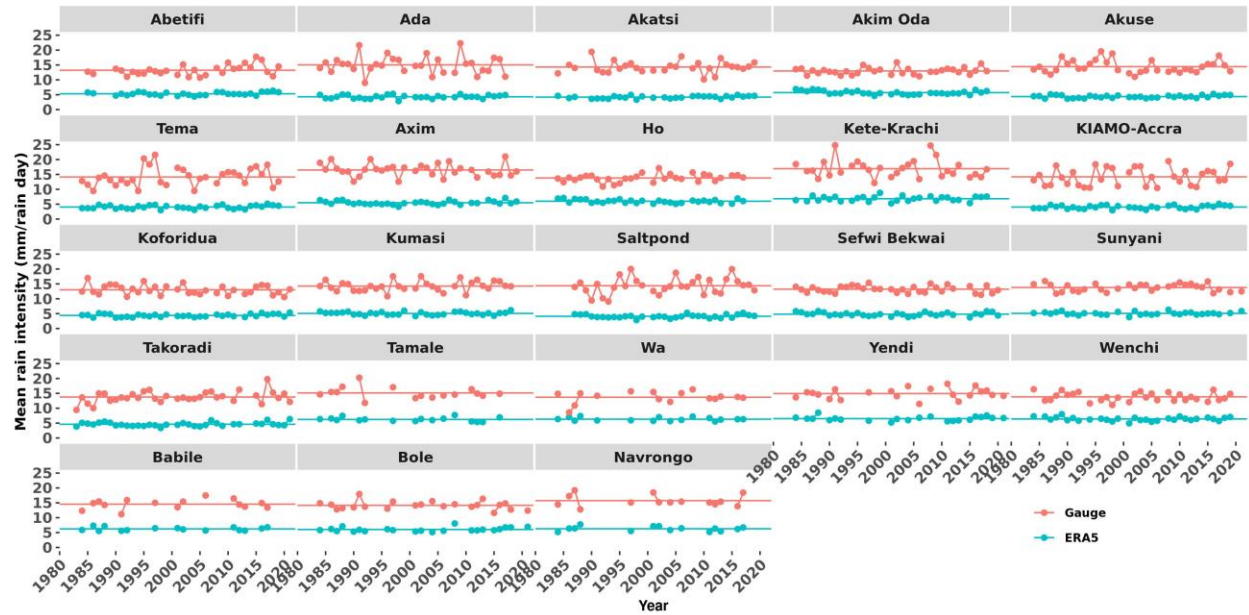

**Fig E67: Mean rain per rainy day across the stations in Ghana – rain gauge vs ERA5. The horizontal lines represent the average mean rain per rainy day across all the years considered for the gauge (red) and the ERA5 (blue)**

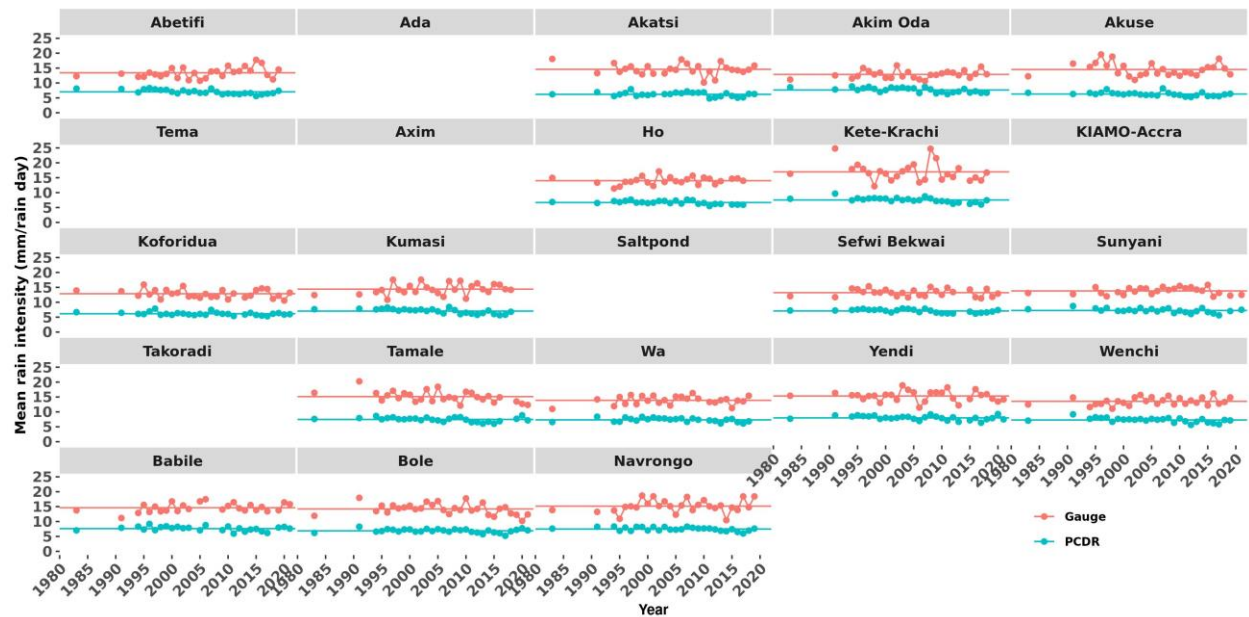

**Fig E68: Mean rain per rainy day across the stations in Ghana – rain gauge vs PCDR. The horizontal lines represent the average mean rain per rainy day across all the years considered for the gauge (red) and the PCDR (blue)**

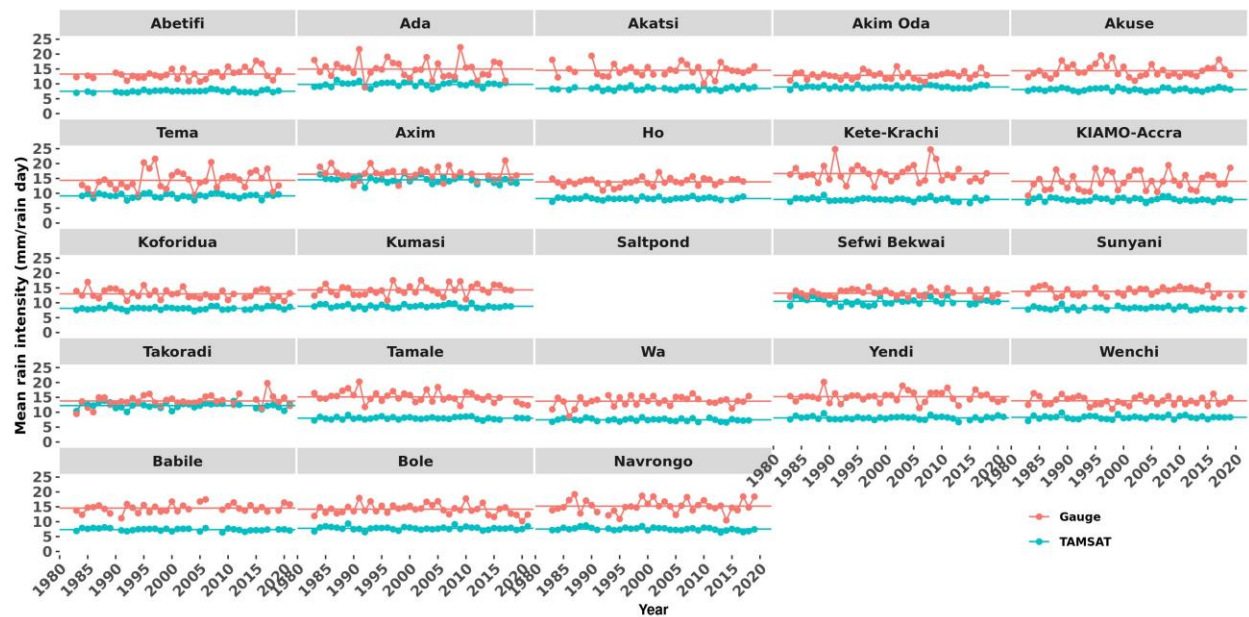

**Fig E69: Mean rain per rainy day across the stations in Ghana – rain gauge vs TAMSAT.** The horizontal lines represent the average mean rain per rainy day across all the years considered for the gauge (red) and the TAMSAT (blue)

**Table E6: Summary statistics on the performance of the products on mean rain per rainy day at the various stations in Ghana**

| metric | station  | CHIRPS | CHIRP | ERA5  | TAMSAT | AGERA5 | PCDR  |
|--------|----------|--------|-------|-------|--------|--------|-------|
| r      | Abetifi  | -0.1   | -0.27 | 0.01  | -0.03  | 0.18   | -0.28 |
| r      | Ada      | 0.28   | 0.34  | 0.32  | 0.18   | 0.21   | NA    |
| r      | Akatsi   | -0.13  | -0.17 | -0.11 | -0.07  | -0.19  | 0.14  |
| r      | Akim Oda | 0.17   | 0.15  | 0.17  | 0.23   | 0.2    | -0.17 |
| r      | Akuse    | 0.39   | 0.14  | -0.07 | 0.28   | -0.03  | 0.1   |
| r      | Tema     | 0.43   | 0.17  | 0.39  | 0.27   | 0.37   | NA    |
| r      | Axim     | 0.09   | 0.31  | 0.34  | 0.24   | 0.32   | NA    |

|              |              |       |       |       |       |       |       |
|--------------|--------------|-------|-------|-------|-------|-------|-------|
| r            | Ho           | 0.08  | -0.03 | 0     | 0.37  | -0.06 | 0.05  |
| r            | Kete-Krachi  | 0.31  | 0.3   | 0.21  | 0.19  | 0.18  | 0.41  |
| r            | KIAMO-Accra  | 0.44  | 0.07  | 0.18  | 0.43  | 0.17  | NA    |
| r            | Koforidua    | 0.25  | 0.23  | 0.11  | 0.21  | 0.09  | -0.01 |
| r            | Kumasi       | 0.14  | 0.04  | 0.18  | 0.15  | 0.24  | -0.19 |
| r            | Saltpond     | 0.43  | 0.05  | -0.01 | NA    | 0.03  | NA    |
| r            | Sefwi Bekwai | -0.07 | -0.06 | -0.06 | 0.02  | 0.04  | 0.04  |
| r            | Sunyani      | 0.16  | 0.14  | -0.11 | -0.01 | -0.08 | -0.1  |
| r            | Takoradi     | 0.17  | 0.12  | 0.32  | 0.17  | 0.33  | NA    |
| r            | Tamale       | 0.42  | 0.04  | 0.01  | 0.2   | -0.04 | 0.11  |
| r            | Wa           | 0.06  | -0.04 | 0     | -0.08 | 0.16  | 0.27  |
| r            | Yendi        | 0.3   | 0.16  | 0.02  | 0.5   | 0.04  | 0.23  |
| r            | Wenchi       | 0.4   | 0.31  | 0.39  | 0.35  | 0.44  | 0.2   |
| r            | Babile       | -0.17 | -0.16 | 0.08  | -0.08 | 0.1   | -0.11 |
| r            | Bole         | 0     | -0.03 | -0.11 | 0.11  | 0.13  | 0.18  |
| r            | Navrongo     | 0.27  | 0.03  | 0.14  | 0.21  | 0.35  | 0.24  |
| <b>PBIAS</b> | Abetifi      | -2    | -59   | -60   | -43   | -60   | -48   |

|              |              |     |     |     |     |     |     |
|--------------|--------------|-----|-----|-----|-----|-----|-----|
| <b>PBIAS</b> | Ada          | -19 | -63 | -71 | -34 | -71 | NA  |
| <b>PBIAS</b> | Akatsi       | -25 | -60 | -71 | -42 | -68 | -58 |
| <b>PBIAS</b> | Akim Oda     | -20 | -55 | -56 | -30 | -58 | -41 |
| <b>PBIAS</b> | Akuse        | -32 | -61 | -70 | -44 | -62 | -57 |
| <b>PBIAS</b> | Tema         | -28 | -63 | -71 | -36 | -72 | NA  |
| <b>PBIAS</b> | Axim         | 13  | -63 | -67 | -12 | -67 | NA  |
| <b>PBIAS</b> | Ho           | -26 | -55 | -57 | -40 | -57 | -52 |
| <b>PBIAS</b> | Kete-Krachi  | -38 | -50 | -60 | -52 | -58 | -56 |
| <b>PBIAS</b> | KIAMO-Accra  | -38 | -62 | -72 | -44 | -71 | NA  |
| <b>PBIAS</b> | Koforidua    | -14 | -54 | -66 | -38 | -61 | -52 |
| <b>PBIAS</b> | Kumasi       | -28 | -58 | -64 | -38 | -66 | -51 |
| <b>PBIAS</b> | Saltpond     | -21 | -66 | -71 | NA  | -71 | NA  |
| <b>PBIAS</b> | Sefwi Bekwai | -1  | -56 | -64 | -21 | -63 | -46 |
| <b>PBIAS</b> | Sunyani      | -30 | -58 | -63 | -41 | -63 | -48 |
| <b>PBIAS</b> | Takoradi     | -11 | -66 | -66 | -11 | -67 | N   |
| <b>PBIAS</b> | Tamale       | -29 | -48 | -59 | -47 | -57 | -51 |
| <b>PBIAS</b> | Wa           | -30 | -48 | -54 | -46 | -52 | -47 |

|              |             |      |      |      |      |      |      |
|--------------|-------------|------|------|------|------|------|------|
| <b>PBIAS</b> | Yendi       | -32  | -47  | -56  | -47  | -56  | -48  |
| <b>PBIAS</b> | Wenchi      | -26  | -51  | -54  | -40  | -53  | -46  |
| <b>PBIAS</b> | Babile      | -37  | -49  | -57  | -50  | -56  | -48  |
| <b>PBIAS</b> | Bole        | -31  | -52  | -57  | -45  | -57  | -52  |
| <b>PBIAS</b> | Navrongo    | -27  | -49  | -60  | -51  | -59  | -51  |
| <b>RSD</b>   | Abetifi     | 0.61 | 0.28 | 0.3  | 0.23 | 0.28 | 0.41 |
| <b>RSD</b>   | Ada         | 0.72 | 0.28 | 0.2  | 0.27 | 0.17 | NA   |
| <b>RSD</b>   | Akatsi      | 0.69 | 0.4  | 0.22 | 0.26 | 0.23 | 0.38 |
| <b>RSD</b>   | Akim Oda    | 0.93 | 0.46 | 0.54 | 0.38 | 0.48 | 0.61 |
| <b>RSD</b>   | Akuse       | 0.52 | 0.36 | 0.22 | 0.23 | 0.25 | 0.3  |
| <b>RSD</b>   | Tema        | 0.56 | 0.32 | 0.19 | 0.23 | 0.19 | NA   |
| <b>RSD</b>   | Axim        | 1.13 | 0.28 | 0.3  | 0.54 | 0.31 | NA   |
| <b>RSD</b>   | Ho          | 0.82 | 0.53 | 0.44 | 0.35 | 0.49 | 0.45 |
| <b>RSD</b>   | Kete-Krachi | 0.39 | 0.48 | 0.28 | 0.19 | 0.32 | 0.26 |
| <b>RSD</b>   | KIAMO-Accra | 0.46 | 0.35 | 0.2  | 0.21 | 0.19 | NA   |
| <b>RSD</b>   | Koforidua   | 0.87 | 0.59 | 0.31 | 0.32 | 0.34 | 0.4  |
| <b>RSD</b>   | Kumasi      | 0.65 | 0.44 | 0.3  | 0.32 | 0.33 | 0.43 |

|            |              |       |       |        |       |        |       |
|------------|--------------|-------|-------|--------|-------|--------|-------|
| <b>RSD</b> | Saltpond     | 0.57  | 0.18  | 0.2    | NA    | 0.19   | NA    |
| <b>RSD</b> | Sefwi Bekwai | 1.23  | 0.61  | 0.52   | 1.0   | 0.52   | 0.46  |
| <b>RSD</b> | Sunyani      | 0.81  | 0.6   | 0.41   | 0.39  | 0.44   | 0.62  |
| <b>RSD</b> | Takoradi     | 0.93  | 0.27  | 0.35   | 0.52  | 0.39   | NA    |
| <b>RSD</b> | Tamale       | 0.65  | 0.57  | 0.36   | 0.23  | 0.52   | 0.38  |
| <b>RSD</b> | Wa           | 0.51  | 0.55  | 0.3    | 0.28  | 0.42   | 0.47  |
| <b>RSD</b> | Yendi        | 0.58  | 0.72  | 0.43   | 0.31  | 0.42   | 0.42  |
| <b>RSD</b> | Wenchi       | 0.71  | 0.66  | 0.44   | 0.4   | 0.47   | 0.59  |
| <b>RSD</b> | Babile       | 0.62  | 0.84  | 0.37   | 0.3   | 0.48   | 0.53  |
| <b>RSD</b> | Bole         | 0.54  | 0.52  | 0.5    | 0.33  | 0.36   | 0.34  |
| <b>RSD</b> | Navrongo     | 0.54  | 0.68  | 0.41   | 0.24  | 0.36   | 0.29  |
| <b>ME</b>  | Abetifi      | -3.54 | -7.85 | -7.92  | -5.76 | -8     | -6.4  |
| <b>ME</b>  | Ada          | -2.82 | -9.39 | -10.72 | -5.13 | -10.6  | NA    |
| <b>ME</b>  | Akatsi       | -3.62 | -8.77 | -10.12 | -6.08 | -9.82  | -8.4  |
| <b>ME</b>  | Akim Oda     | -2.57 | -7.05 | -7.27  | -3.9  | -7.4   | -5.23 |
| <b>ME</b>  | Akuse        | -4.66 | -8.78 | -10.05 | -6.32 | -8.97  | -8.22 |
| <b>ME</b>  | Tema         | -4    | -9.04 | -10.09 | -5.23 | -10.34 | NA    |

|    |              |       |        |        |       |        |       |
|----|--------------|-------|--------|--------|-------|--------|-------|
| ME | Axim         | 2.14  | -10.32 | -10.99 | -1.89 | -11.02 | NA    |
| ME | Ho           | -3.65 | -7.57  | -7.81  | -5.6  | -7.86  | -7.33 |
| ME | Kete-Krachi  | -6.41 | -8.32  | -10.09 | -8.71 | -9.73  | -9.42 |
| ME | KIAMO-Accra  | -5.31 | -8.67  | -10.16 | -6.14 | -10.02 | NA    |
| ME | Koforidua    | -1.84 | -6.95  | -8.62  | -4.87 | -7.88  | -6.71 |
| ME | Kumasi       | -4.06 | -8.28  | -9.19  | -5.51 | -9.47  | -7.37 |
| ME | Saltpond     | -2.91 | -9.3   | -10.26 | NA    | -10.06 | NA    |
| ME | Sefwi Bekwai | -0.12 | -7.4   | -8.4   | -2.73 | -8.38  | -6.13 |
| ME | Sunyani      | -4.1  | -8.01  | -8.7   | -5.63 | -8.74  | -6.56 |
| ME | Takoradi     | -1.55 | -9.11  | -9.15  | -1.56 | -9.21  | NA    |
| ME | Tamale       | -4.38 | -7.29  | -8.91  | -7.16 | -8.64  | -7.67 |
| ME | Wa           | -4.1  | -6.6   | -7.37  | -6.26 | -7.2   | -6.56 |
| ME | Yendi        | -4.84 | -7.1   | -8.43  | -7.15 | -8.61  | -7.33 |
| ME | Wenchi       | -3.53 | -7.09  | -7.44  | -5.55 | -7.38  | -6.28 |
| ME | Babile       | -5.37 | -7.15  | -8.33  | -7.23 | -8.2   | -7.01 |
| ME | Bole         | -4.36 | -7.39  | -8.11  | -6.43 | -8.1   | -7.34 |
| ME | Navrongo     | -4.16 | -7.43  | -9.47  | -7.7  | -8.98  | -7.7  |
